# Supplementary material for: Connecting Web Event Forecasting with Anomaly Detection: A Case Study on Enterprise Web Applications Using Self-Supervised Neural Networks
Source: arXiv:2008.13707 source file (2020-09-07)
Supplement: Supplementary file 1 [file appendix.tex]

% \textbf{Model Comparison on Predicting with More Events}

% \subsection{Neural Network Comparison - False Positive}
% We further compare three neural networks in terms of false positive rates. 

\subsection{Evaluation on Predicting Centered Events}
% In addition to Section~\ref{sec:center}, 

\begin{figure*}[!tb]
\centering
\begin{subfigure}{0.32\linewidth}
\centering
\includegraphics[width=0.85\linewidth]{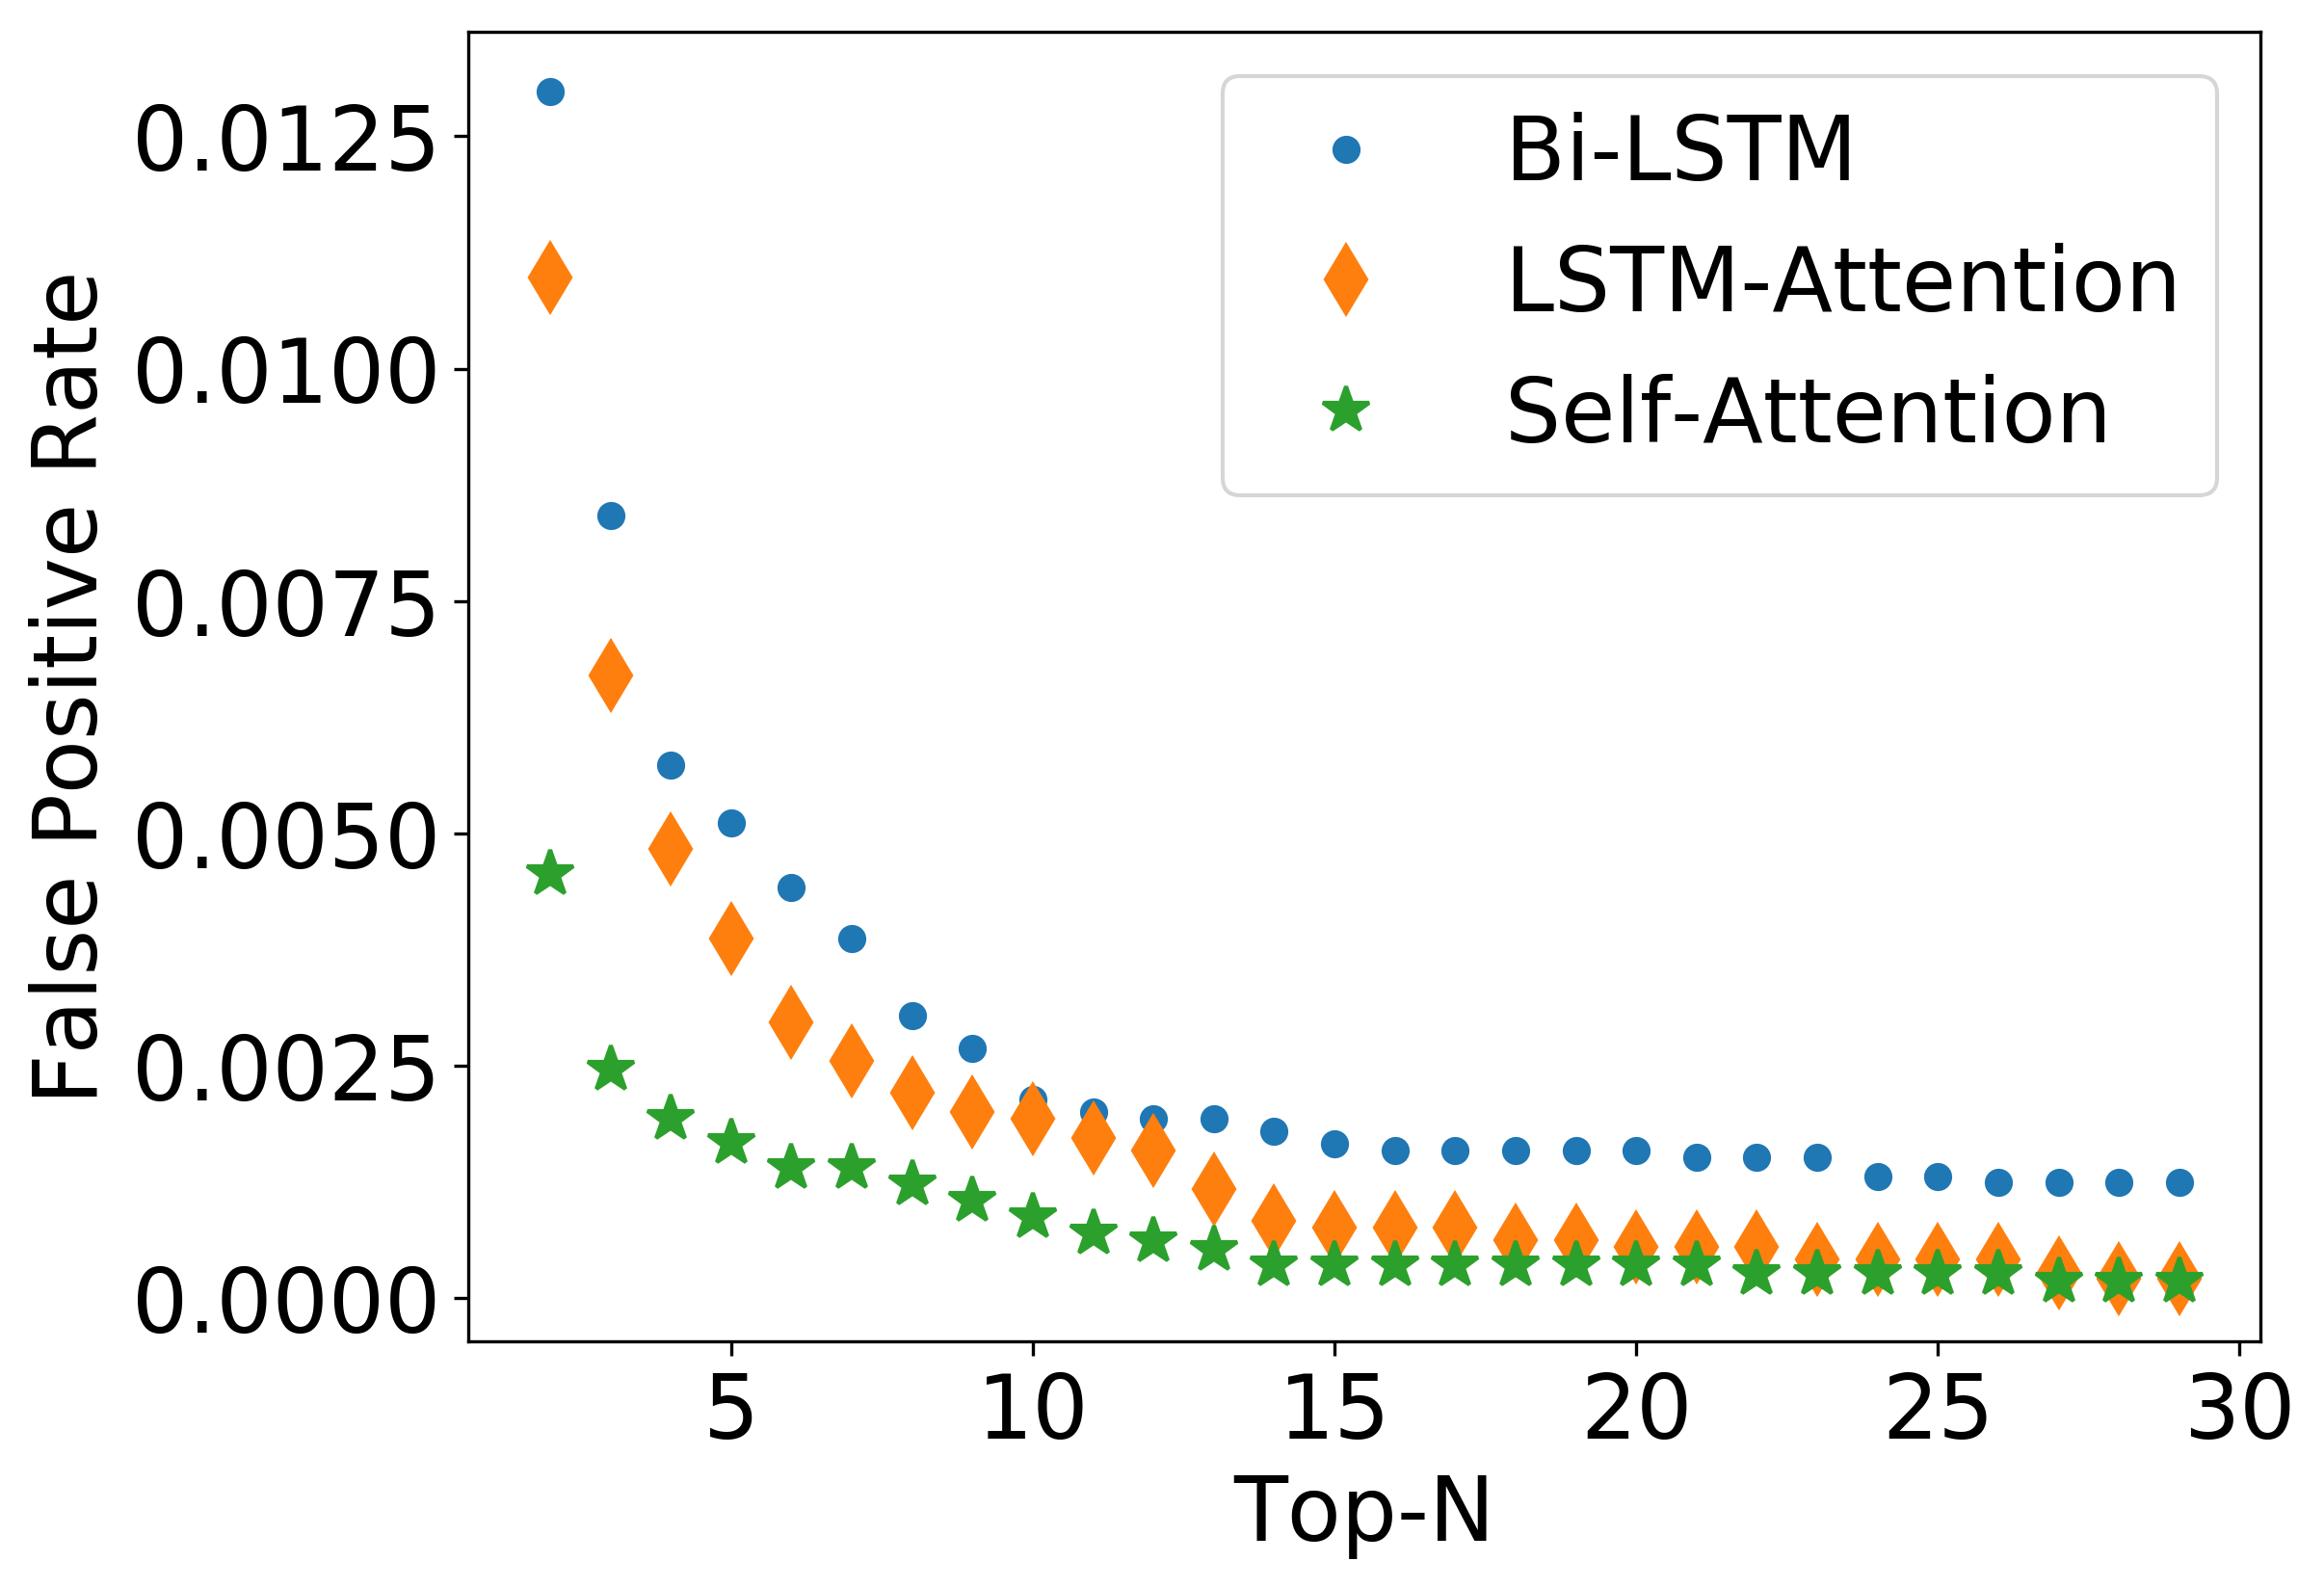}
\caption{Workqueue}
\end{subfigure}
\begin{subfigure}{0.32\linewidth}
\centering
\includegraphics[width=0.85\linewidth]{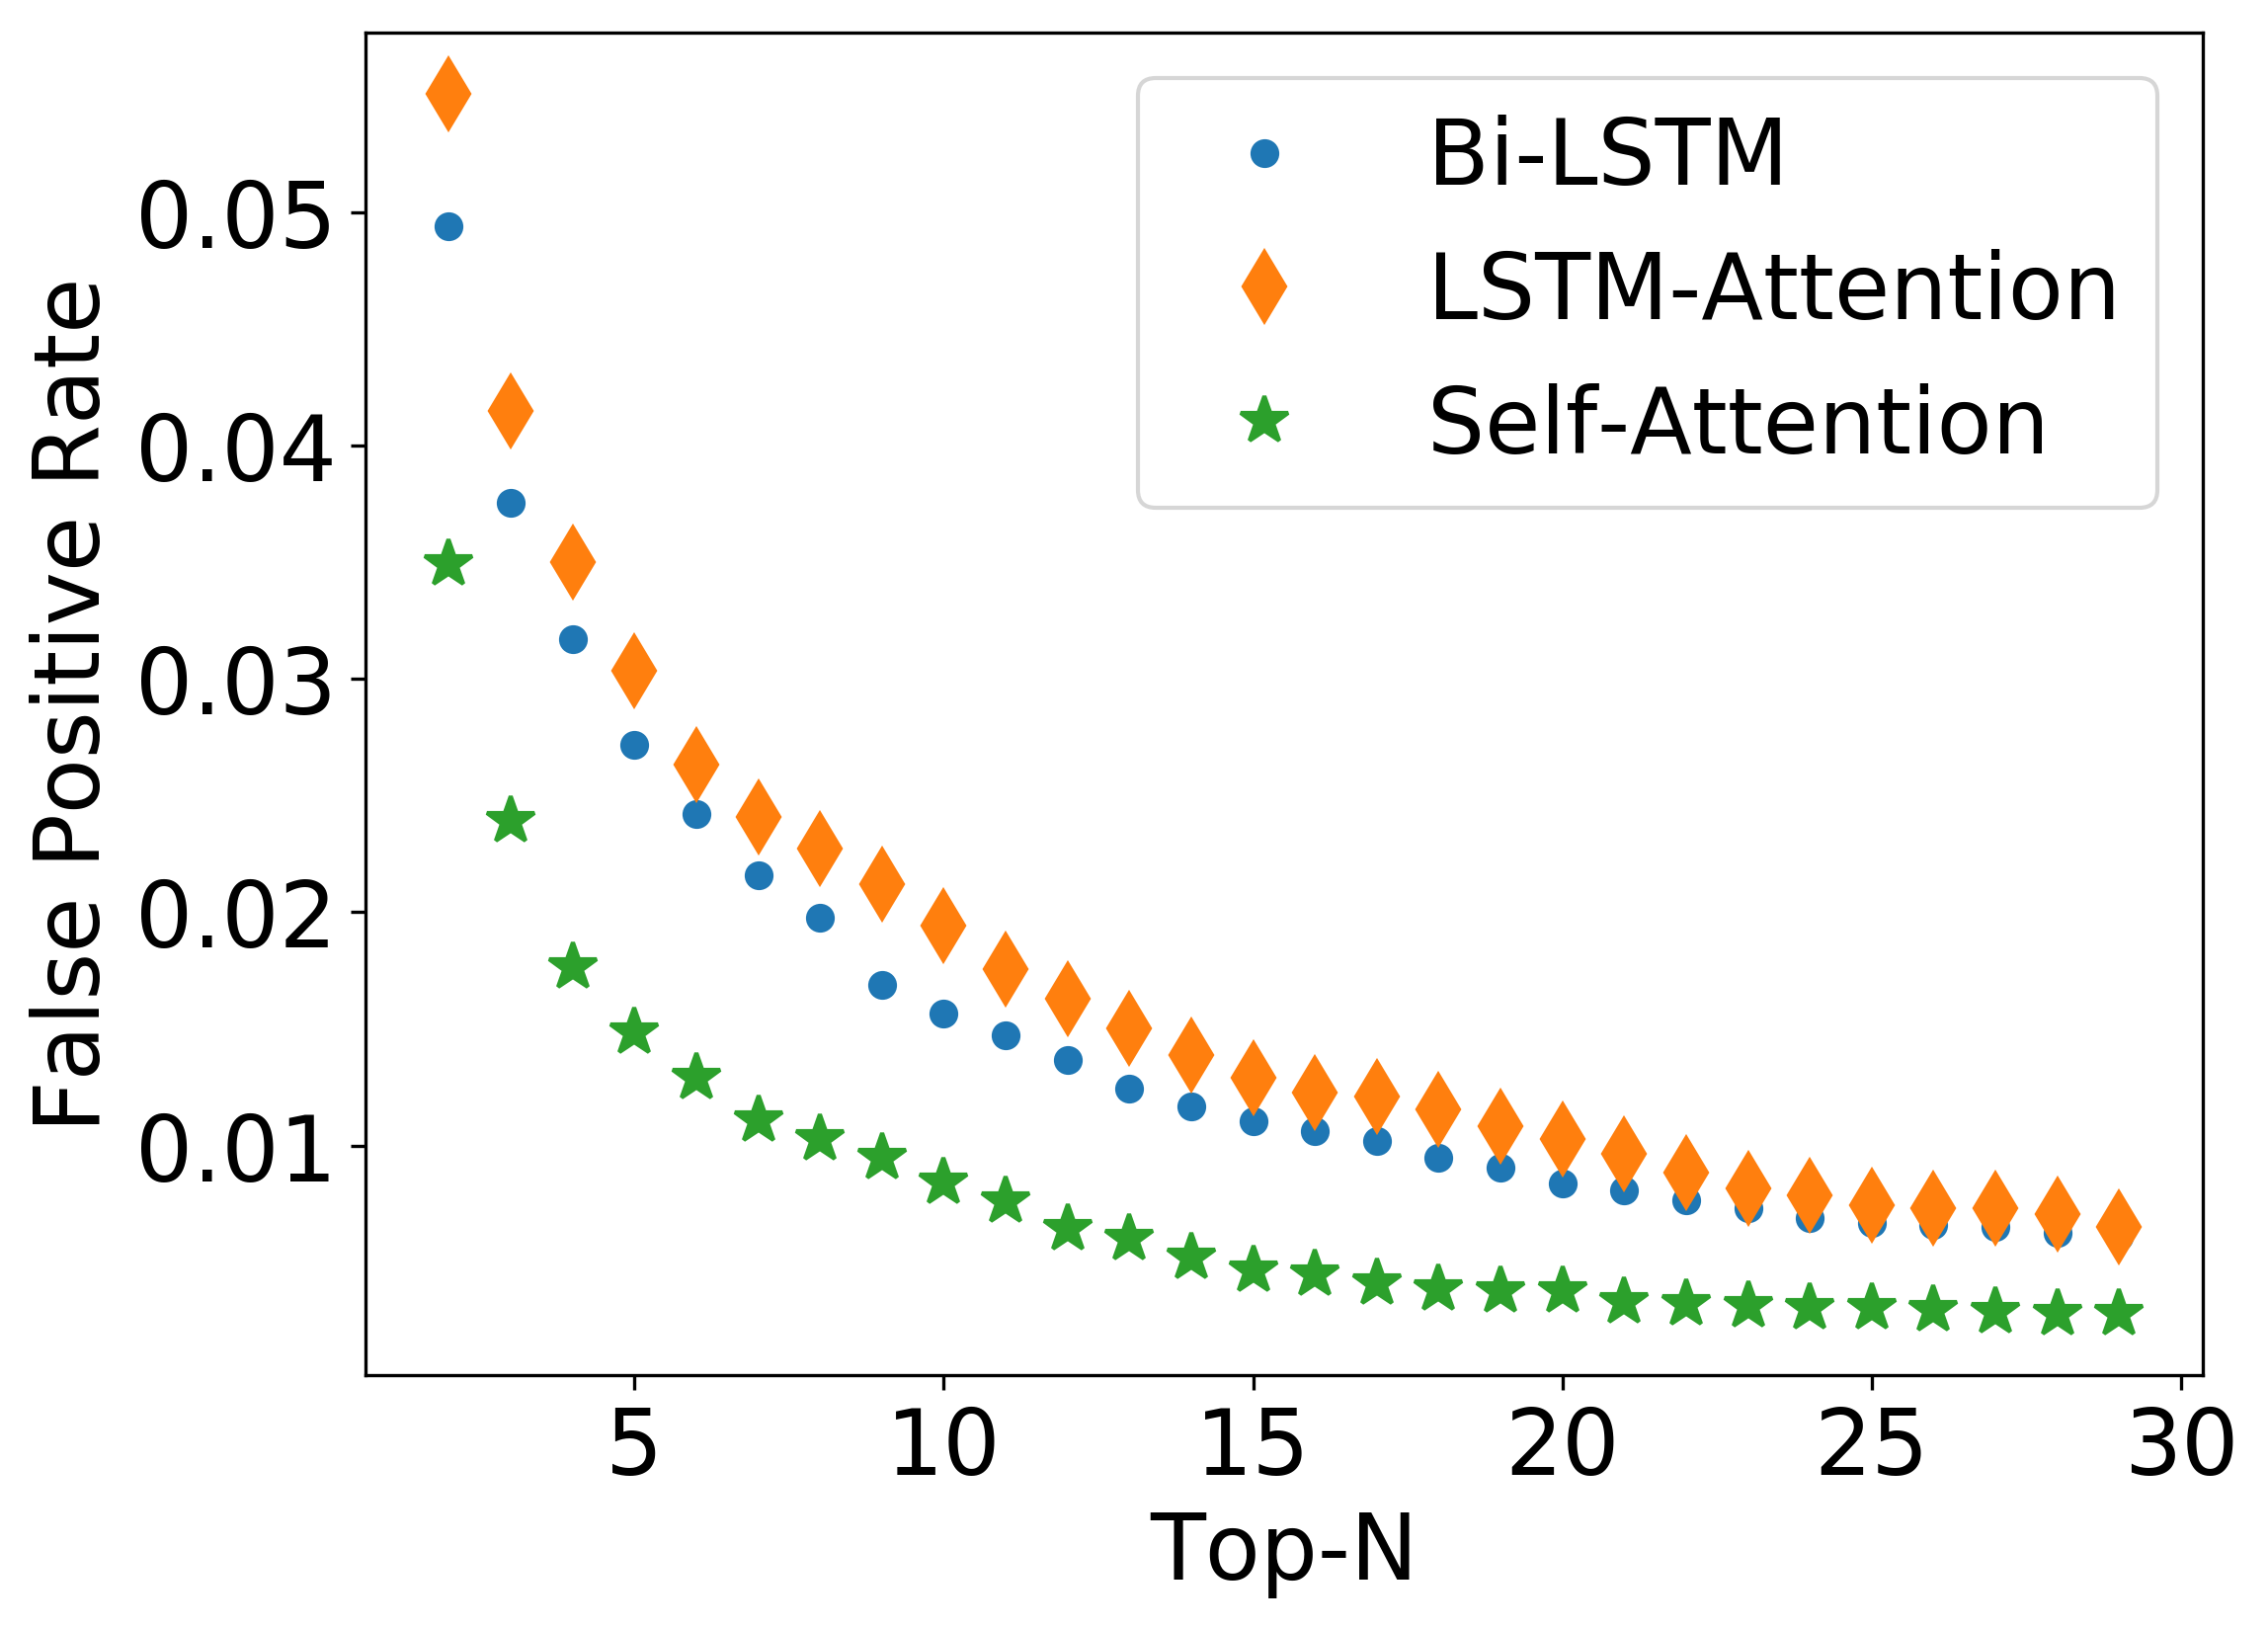}
\caption{DataRepo1}
\end{subfigure}
\begin{subfigure}{0.32\linewidth}
\centering
\includegraphics[width=0.85\linewidth]{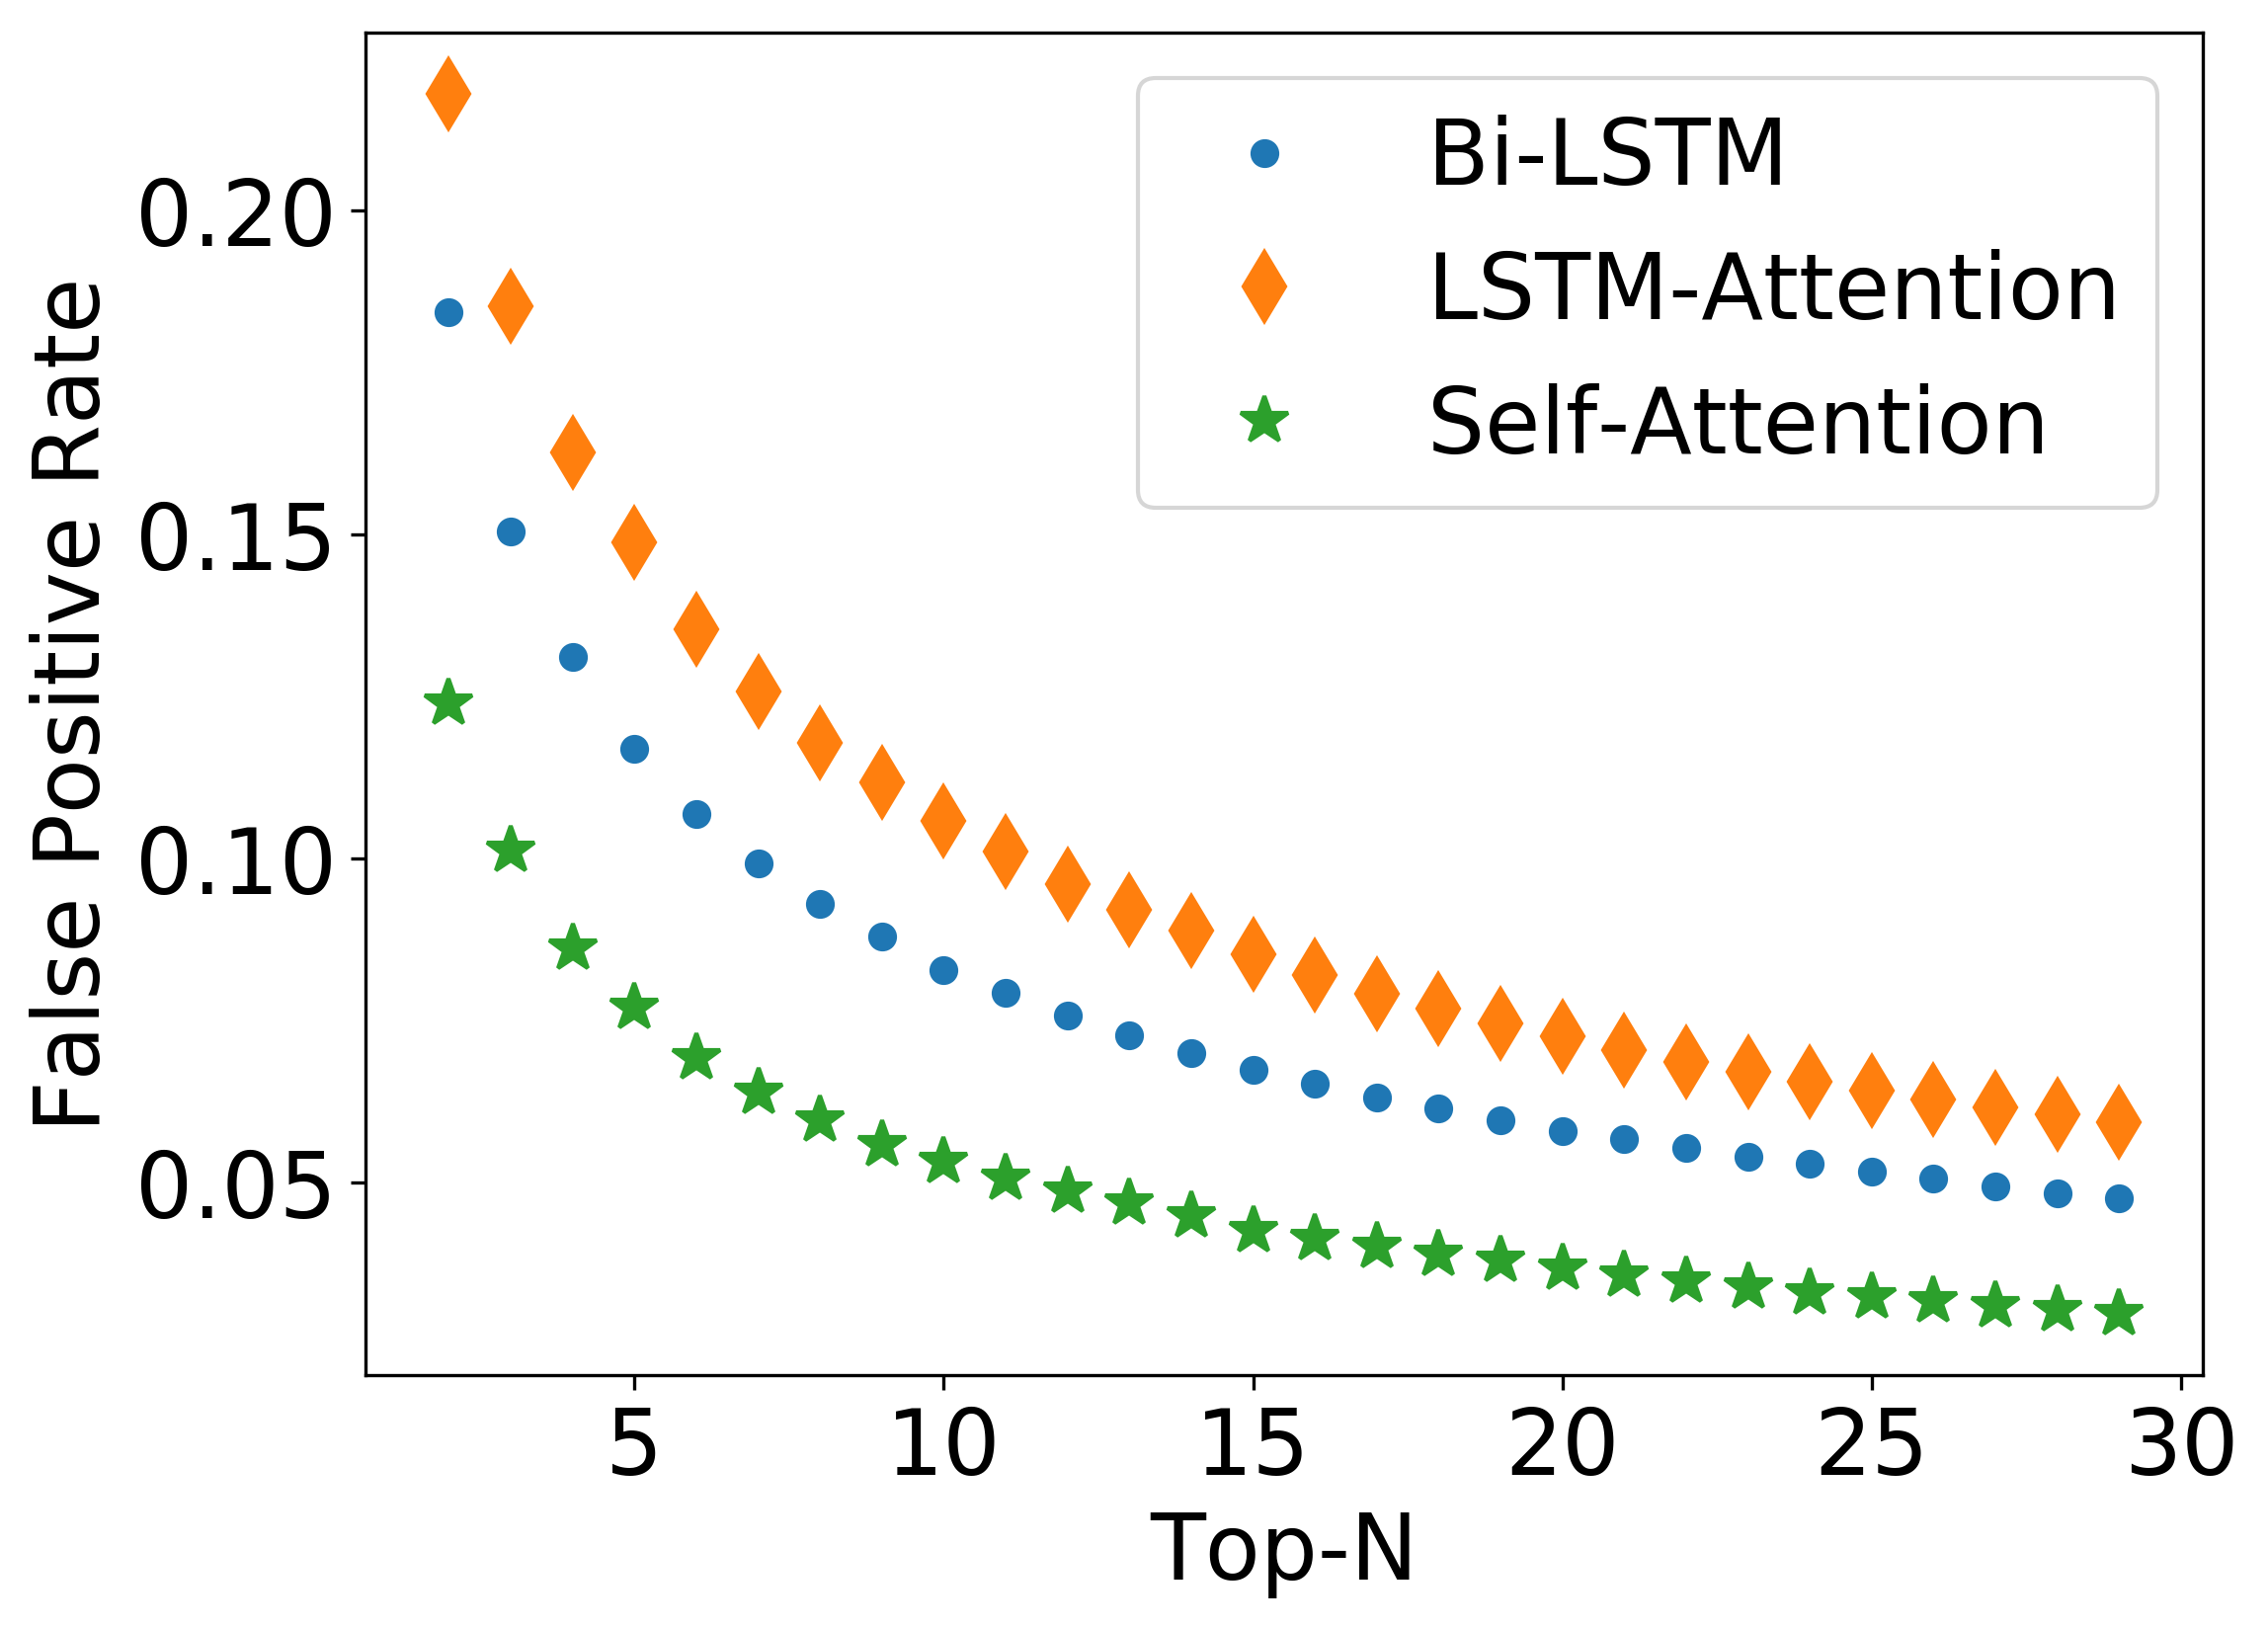}
\caption{DevOpsApp}
\end{subfigure}
\begin{subfigure}{0.32\linewidth}
\centering
\includegraphics[width=0.85\linewidth]{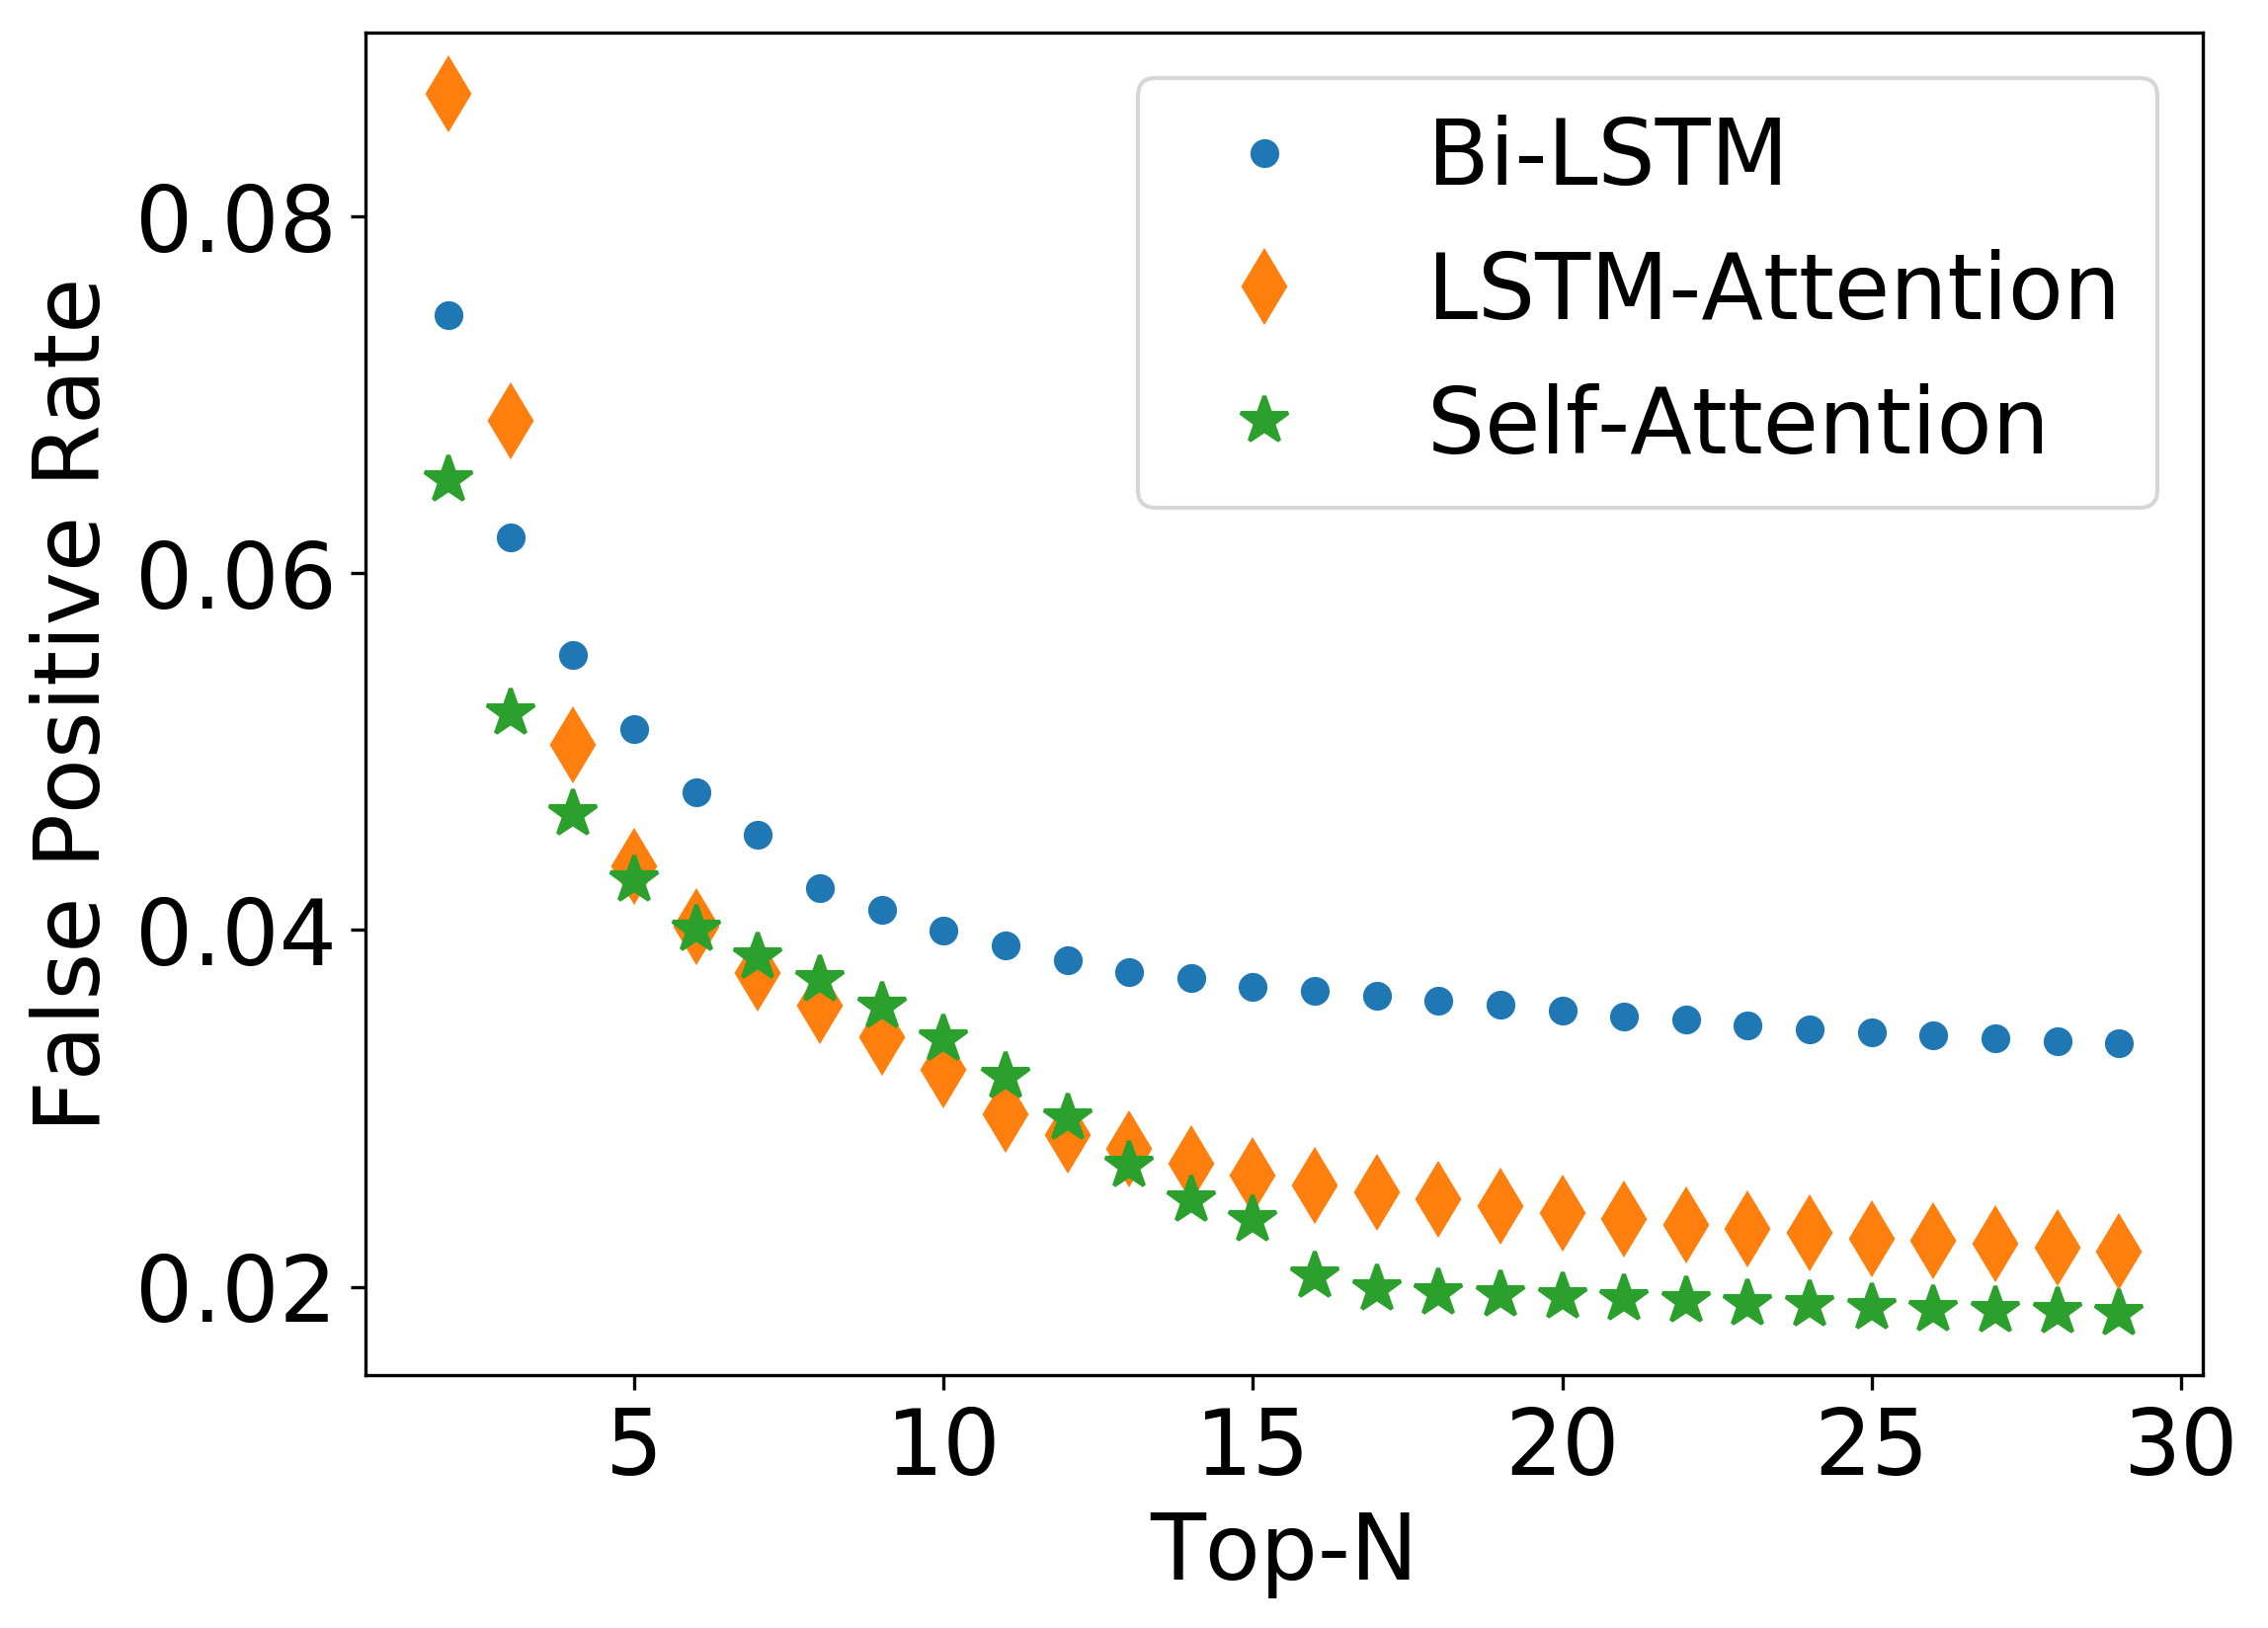}
\caption{DataAnalyzer1}
\end{subfigure}
\begin{subfigure}{0.32\linewidth}
\centering
\includegraphics[width=0.85\linewidth]{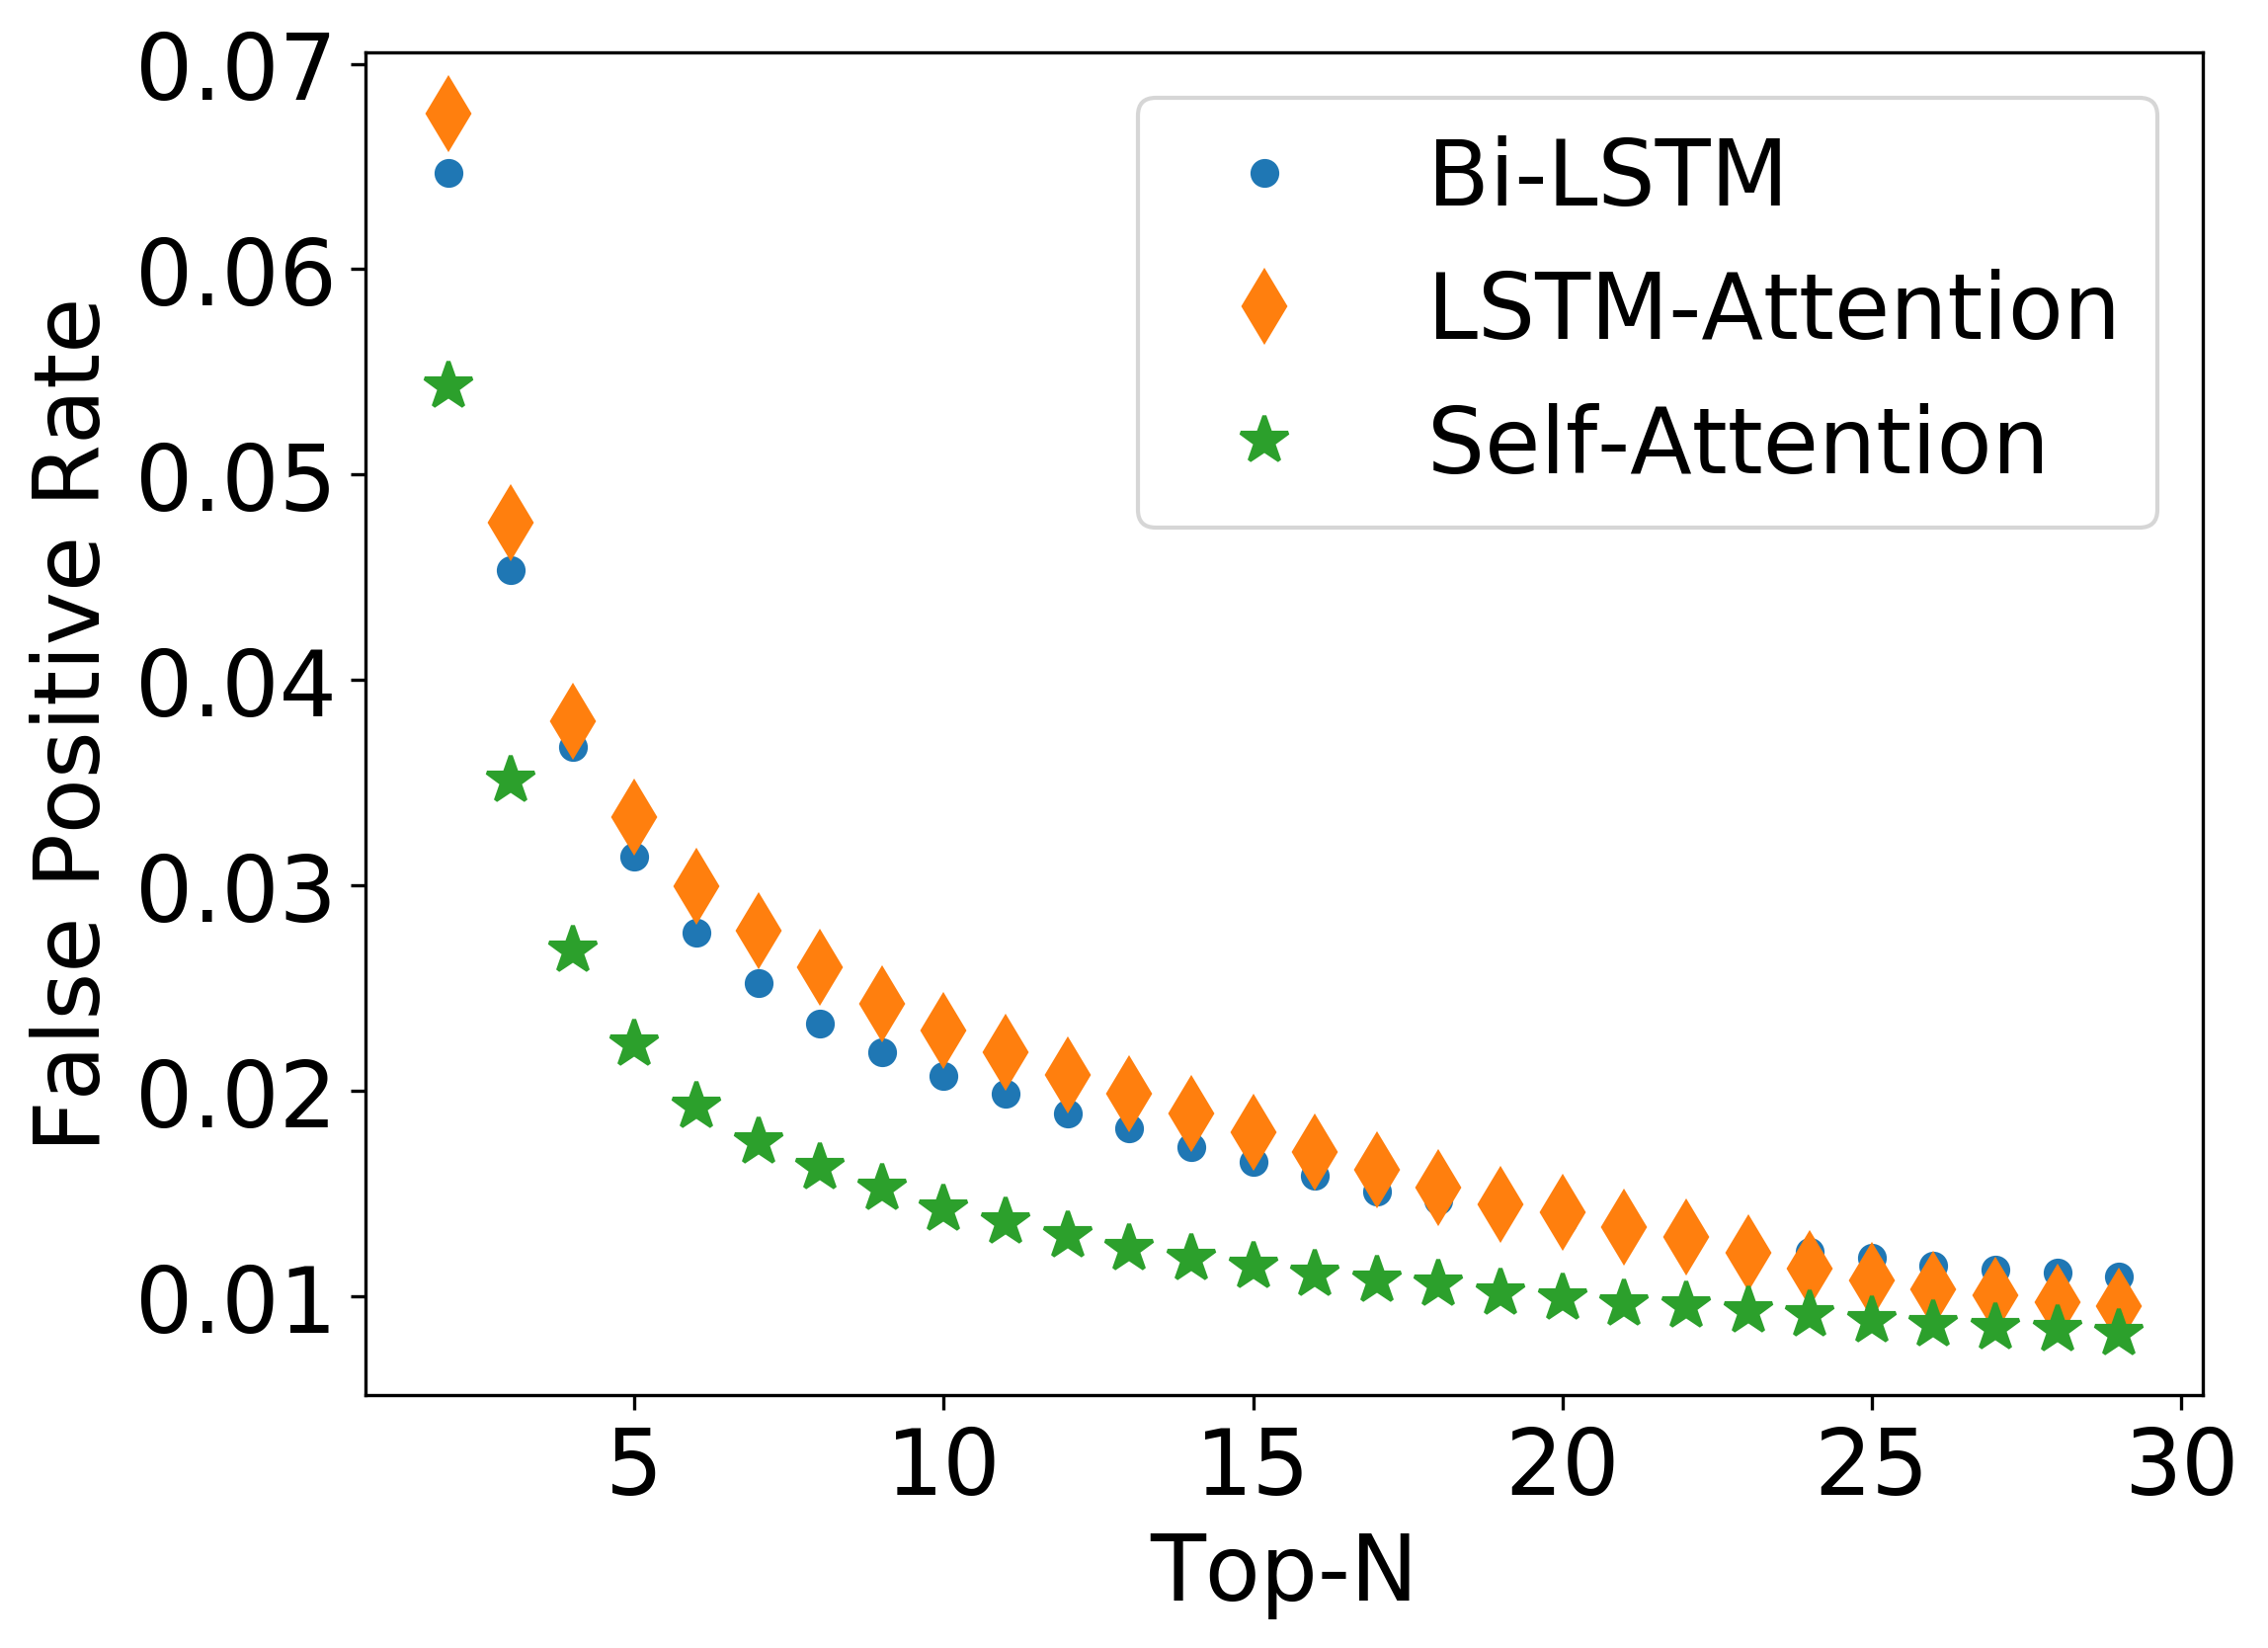}
\caption{DataAnalyzer2}
\end{subfigure}
\begin{subfigure}{0.32\linewidth}
\centering
\includegraphics[width=0.85\linewidth]{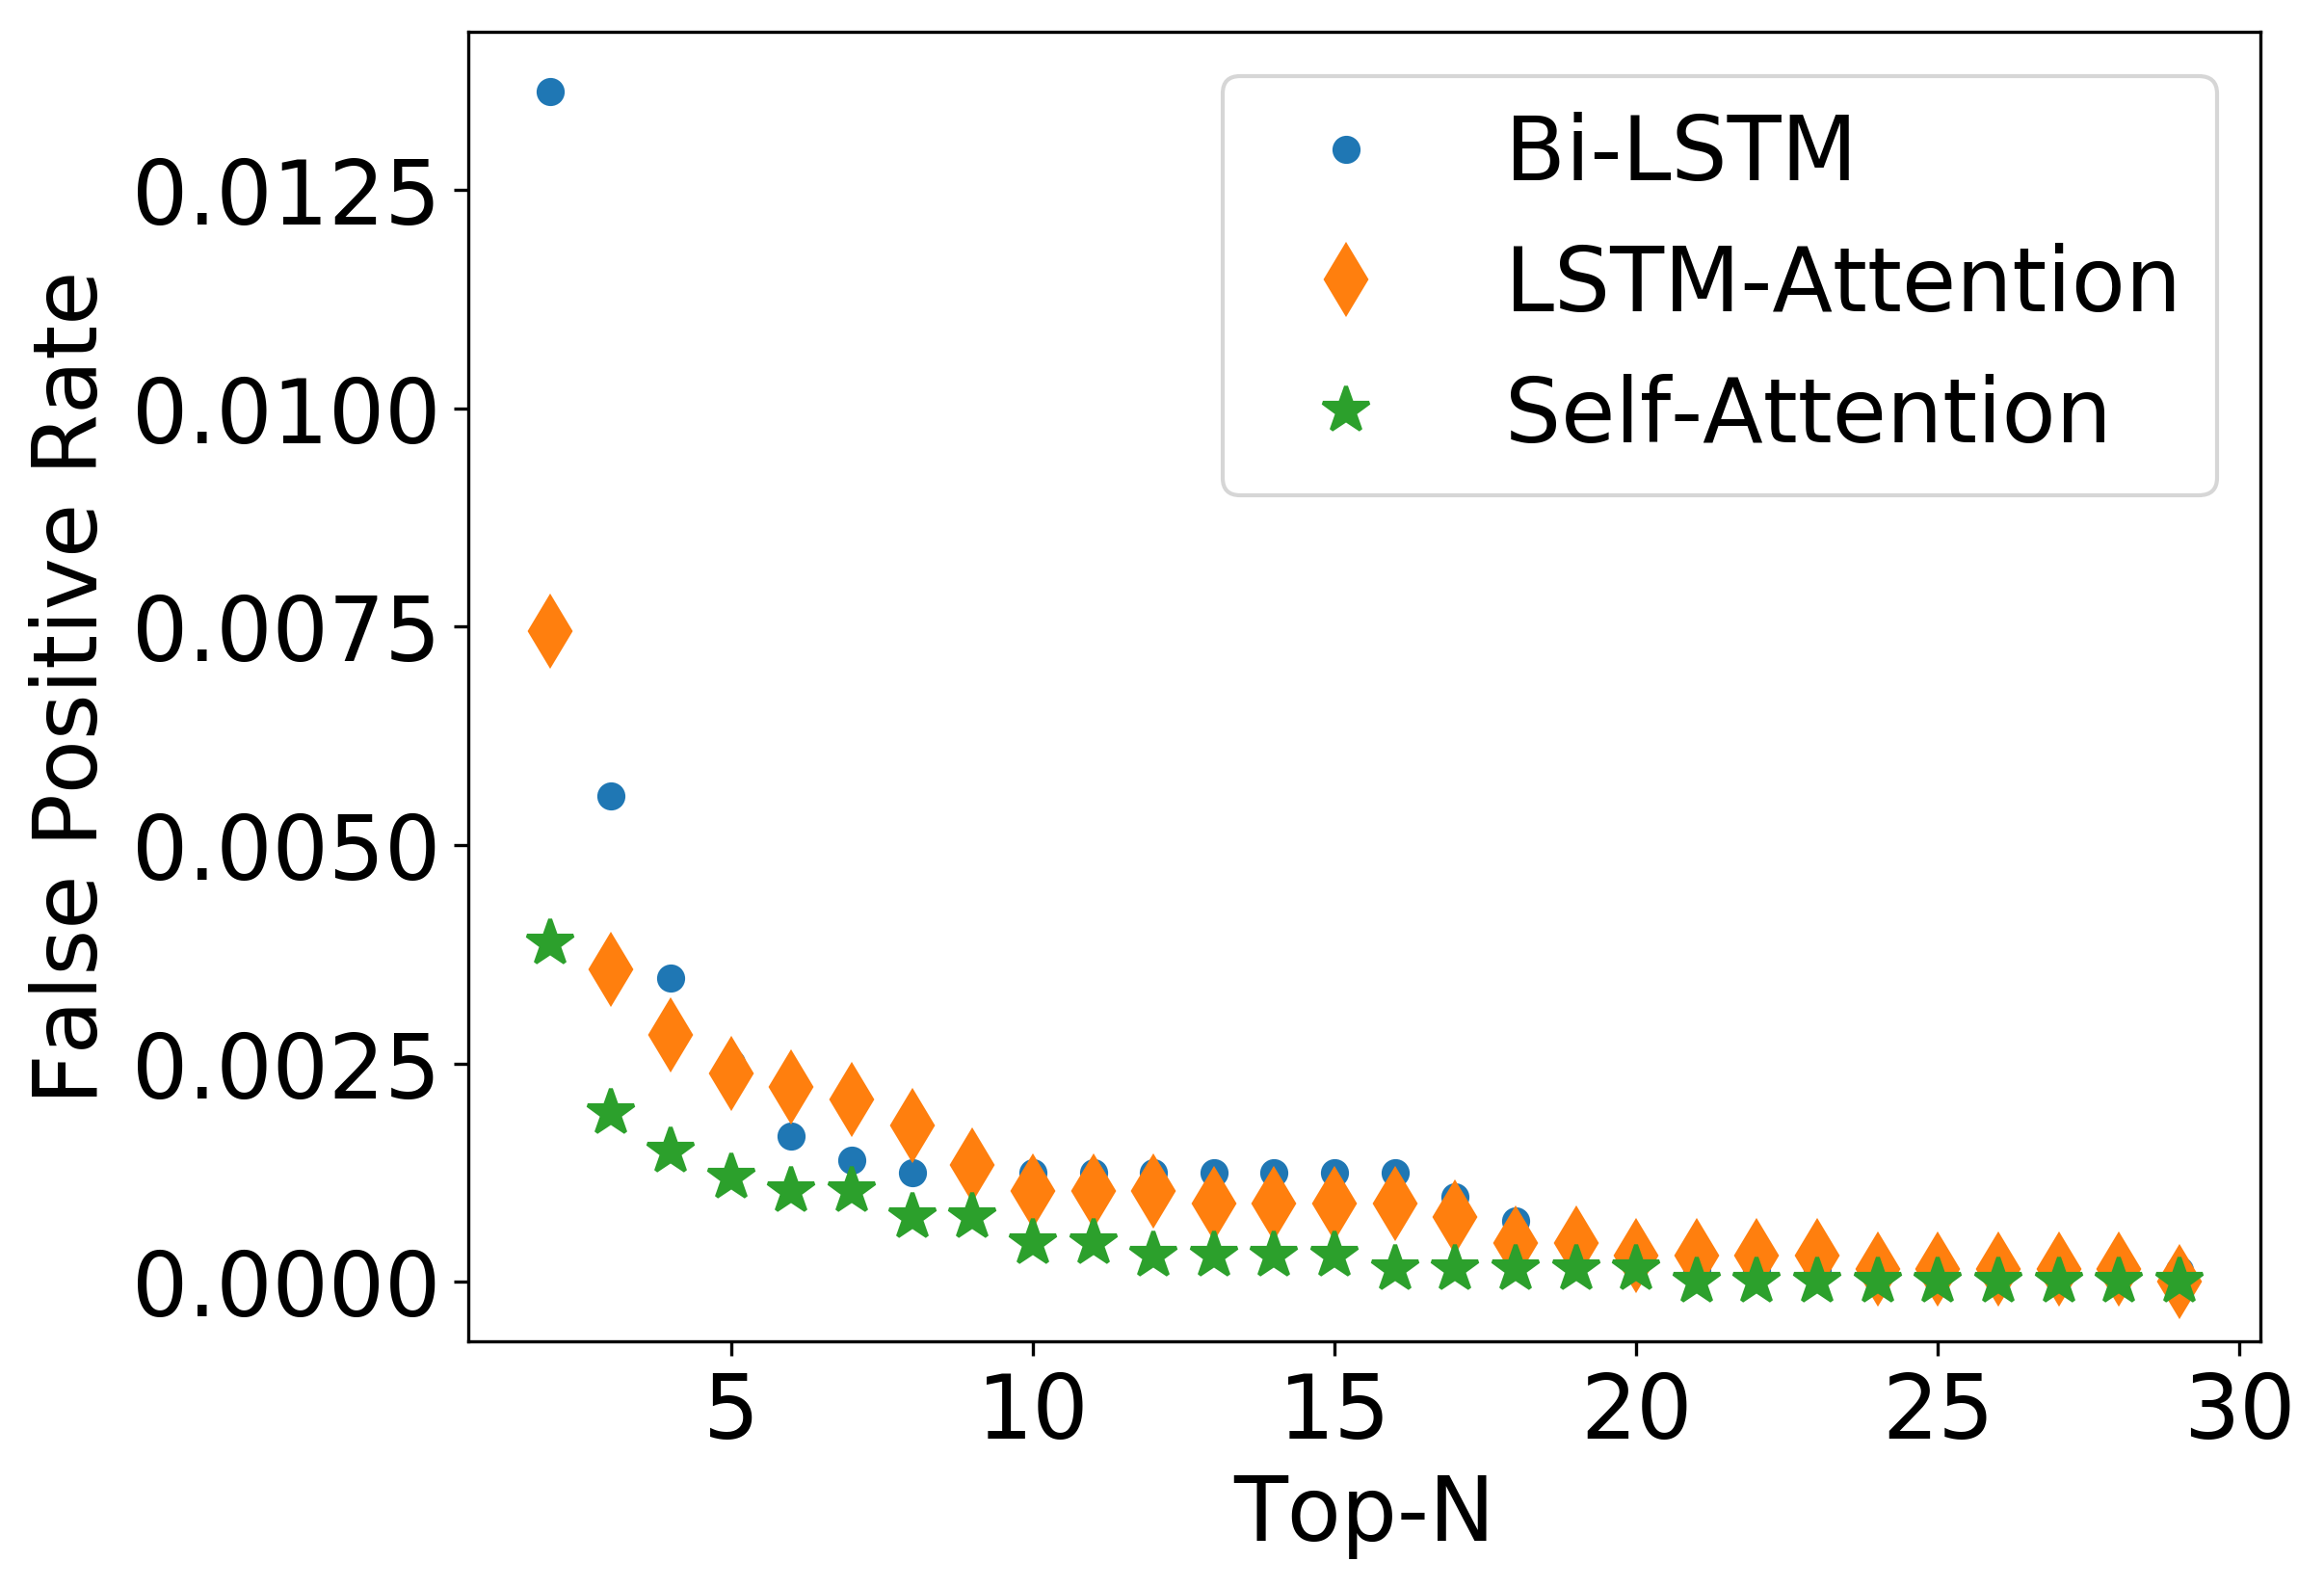}
\caption{DataRepo2}
\end{subfigure}
\caption{False Positive Rate Comparison (Predicting Centered Events).}
\label{fig:fpr_offline}
\end{figure*}

\begin{figure*}[!tb]
\centering
\begin{subfigure}{0.32\linewidth}
\includegraphics[width=0.85\linewidth]{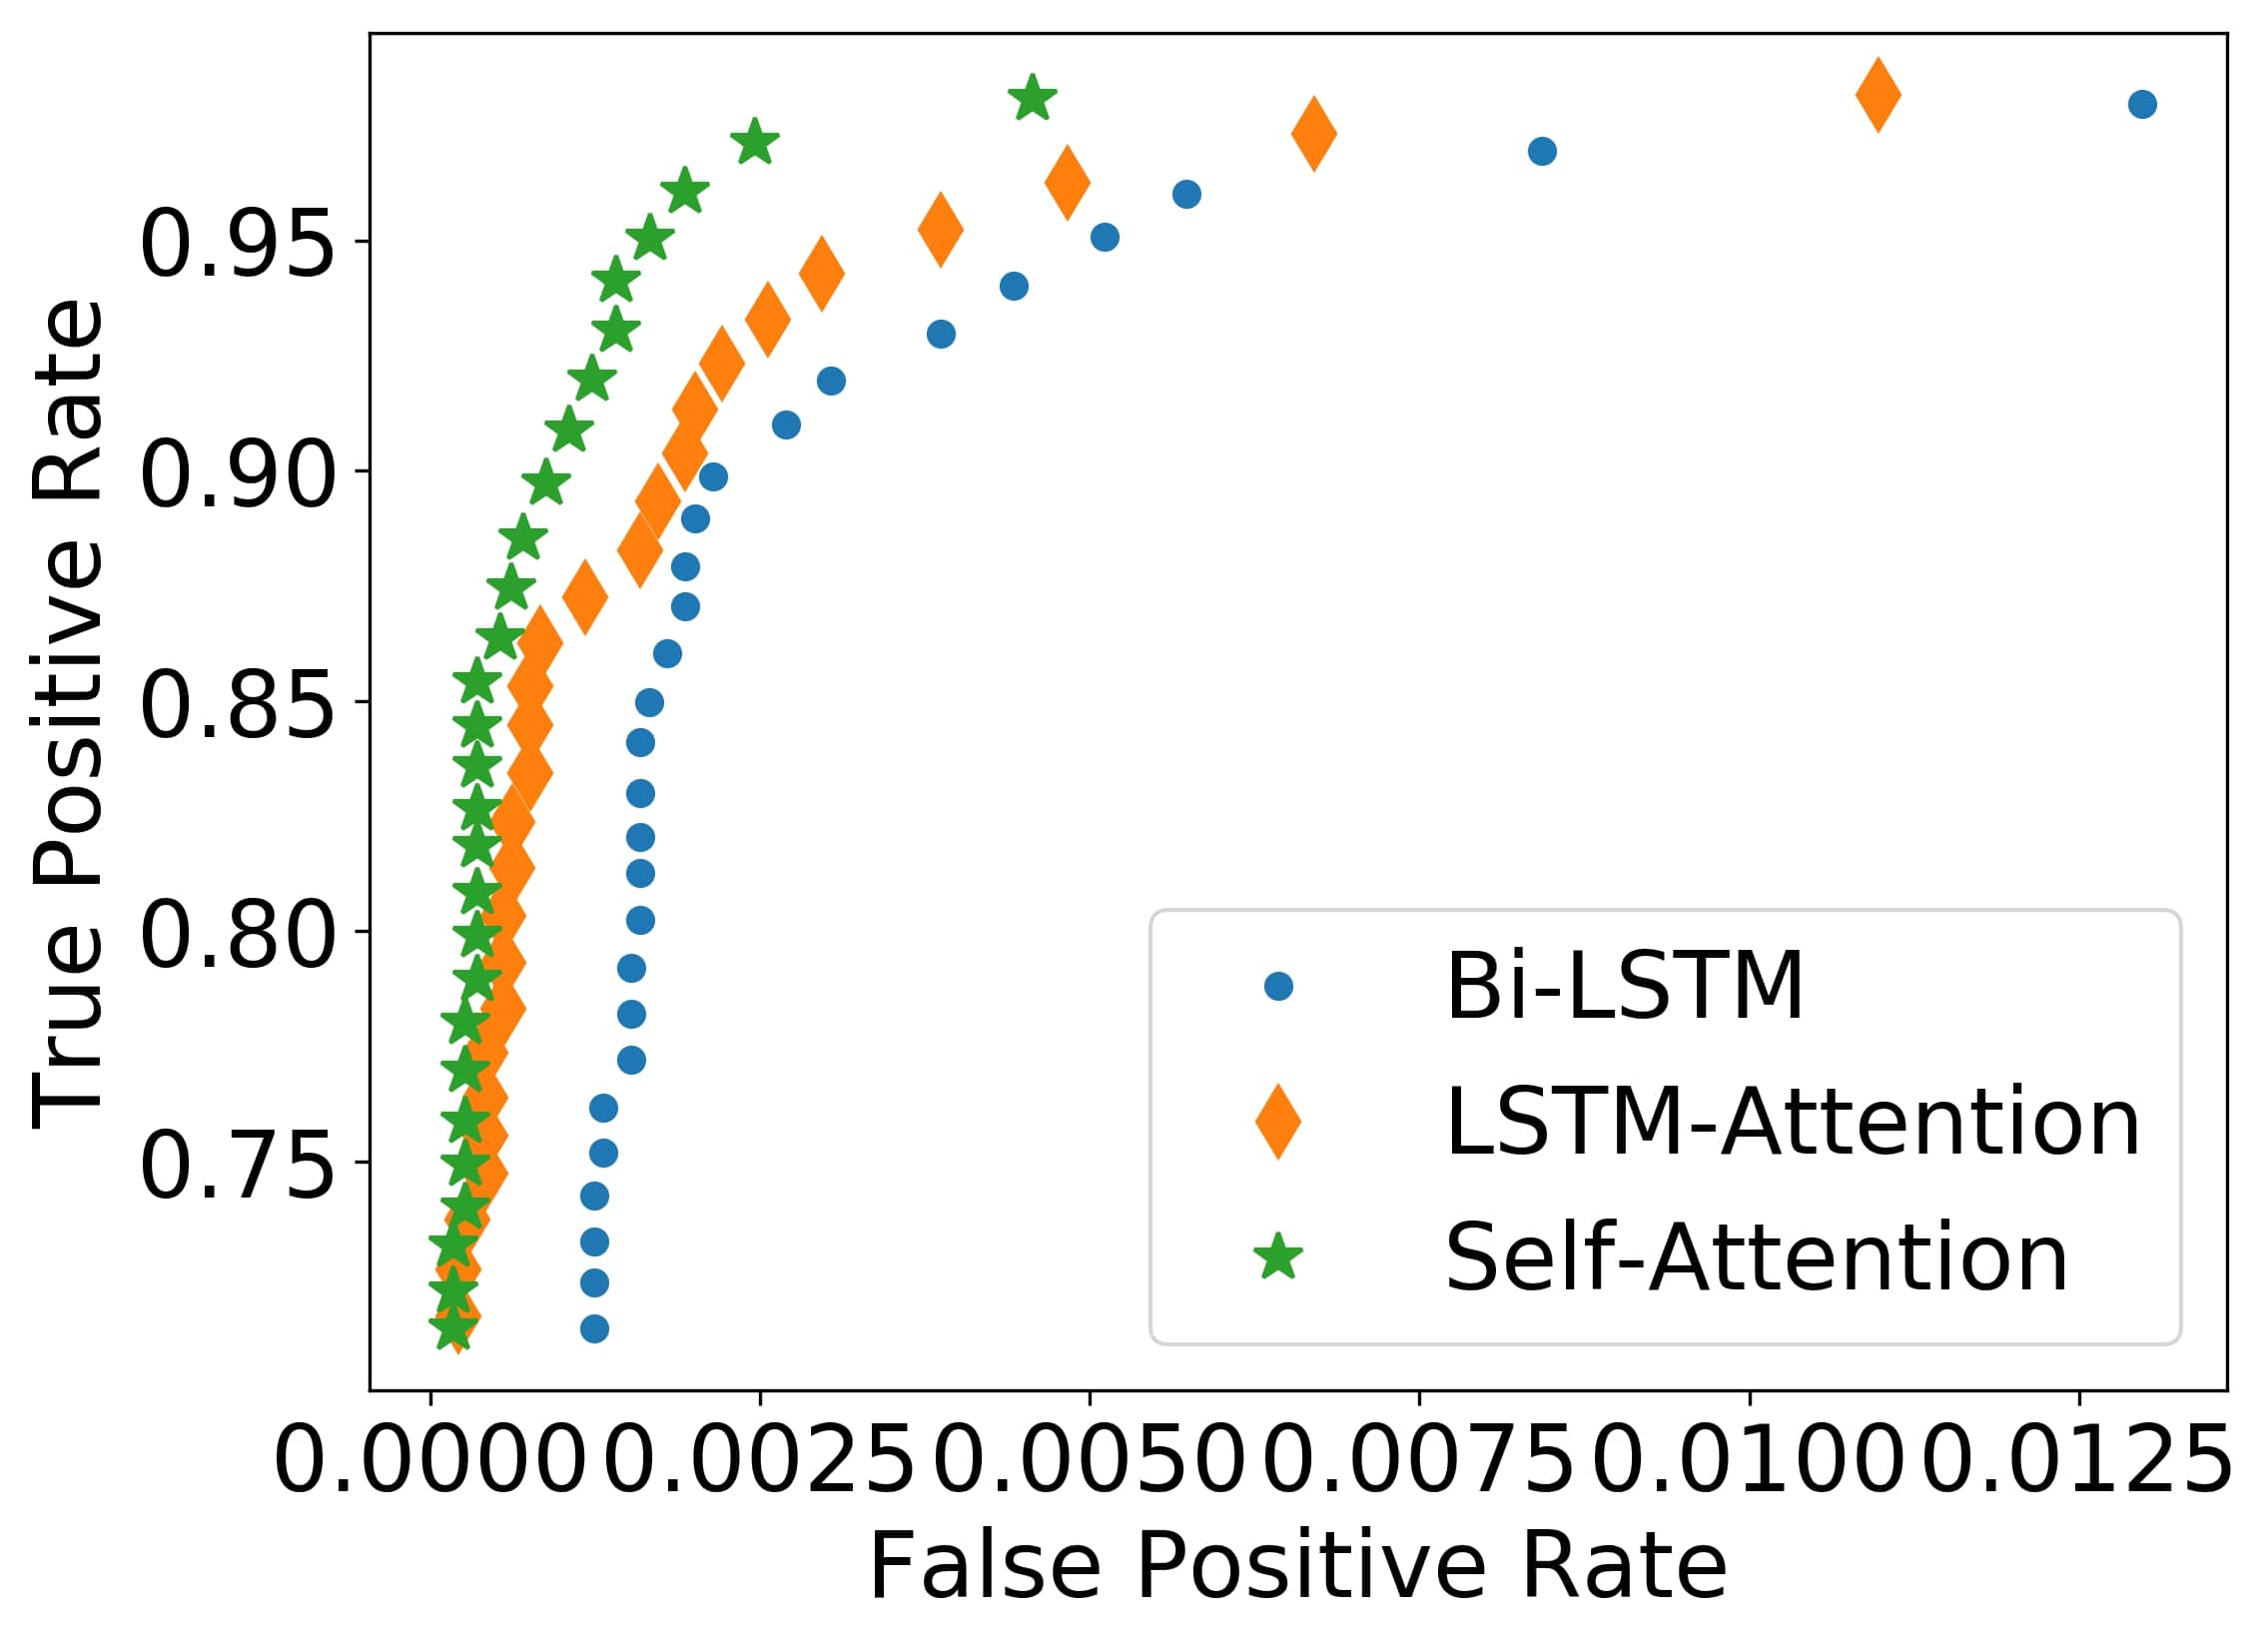}
\caption{Workqueue}
\end{subfigure}
\begin{subfigure}{0.32\linewidth}
\includegraphics[width=0.85\linewidth]{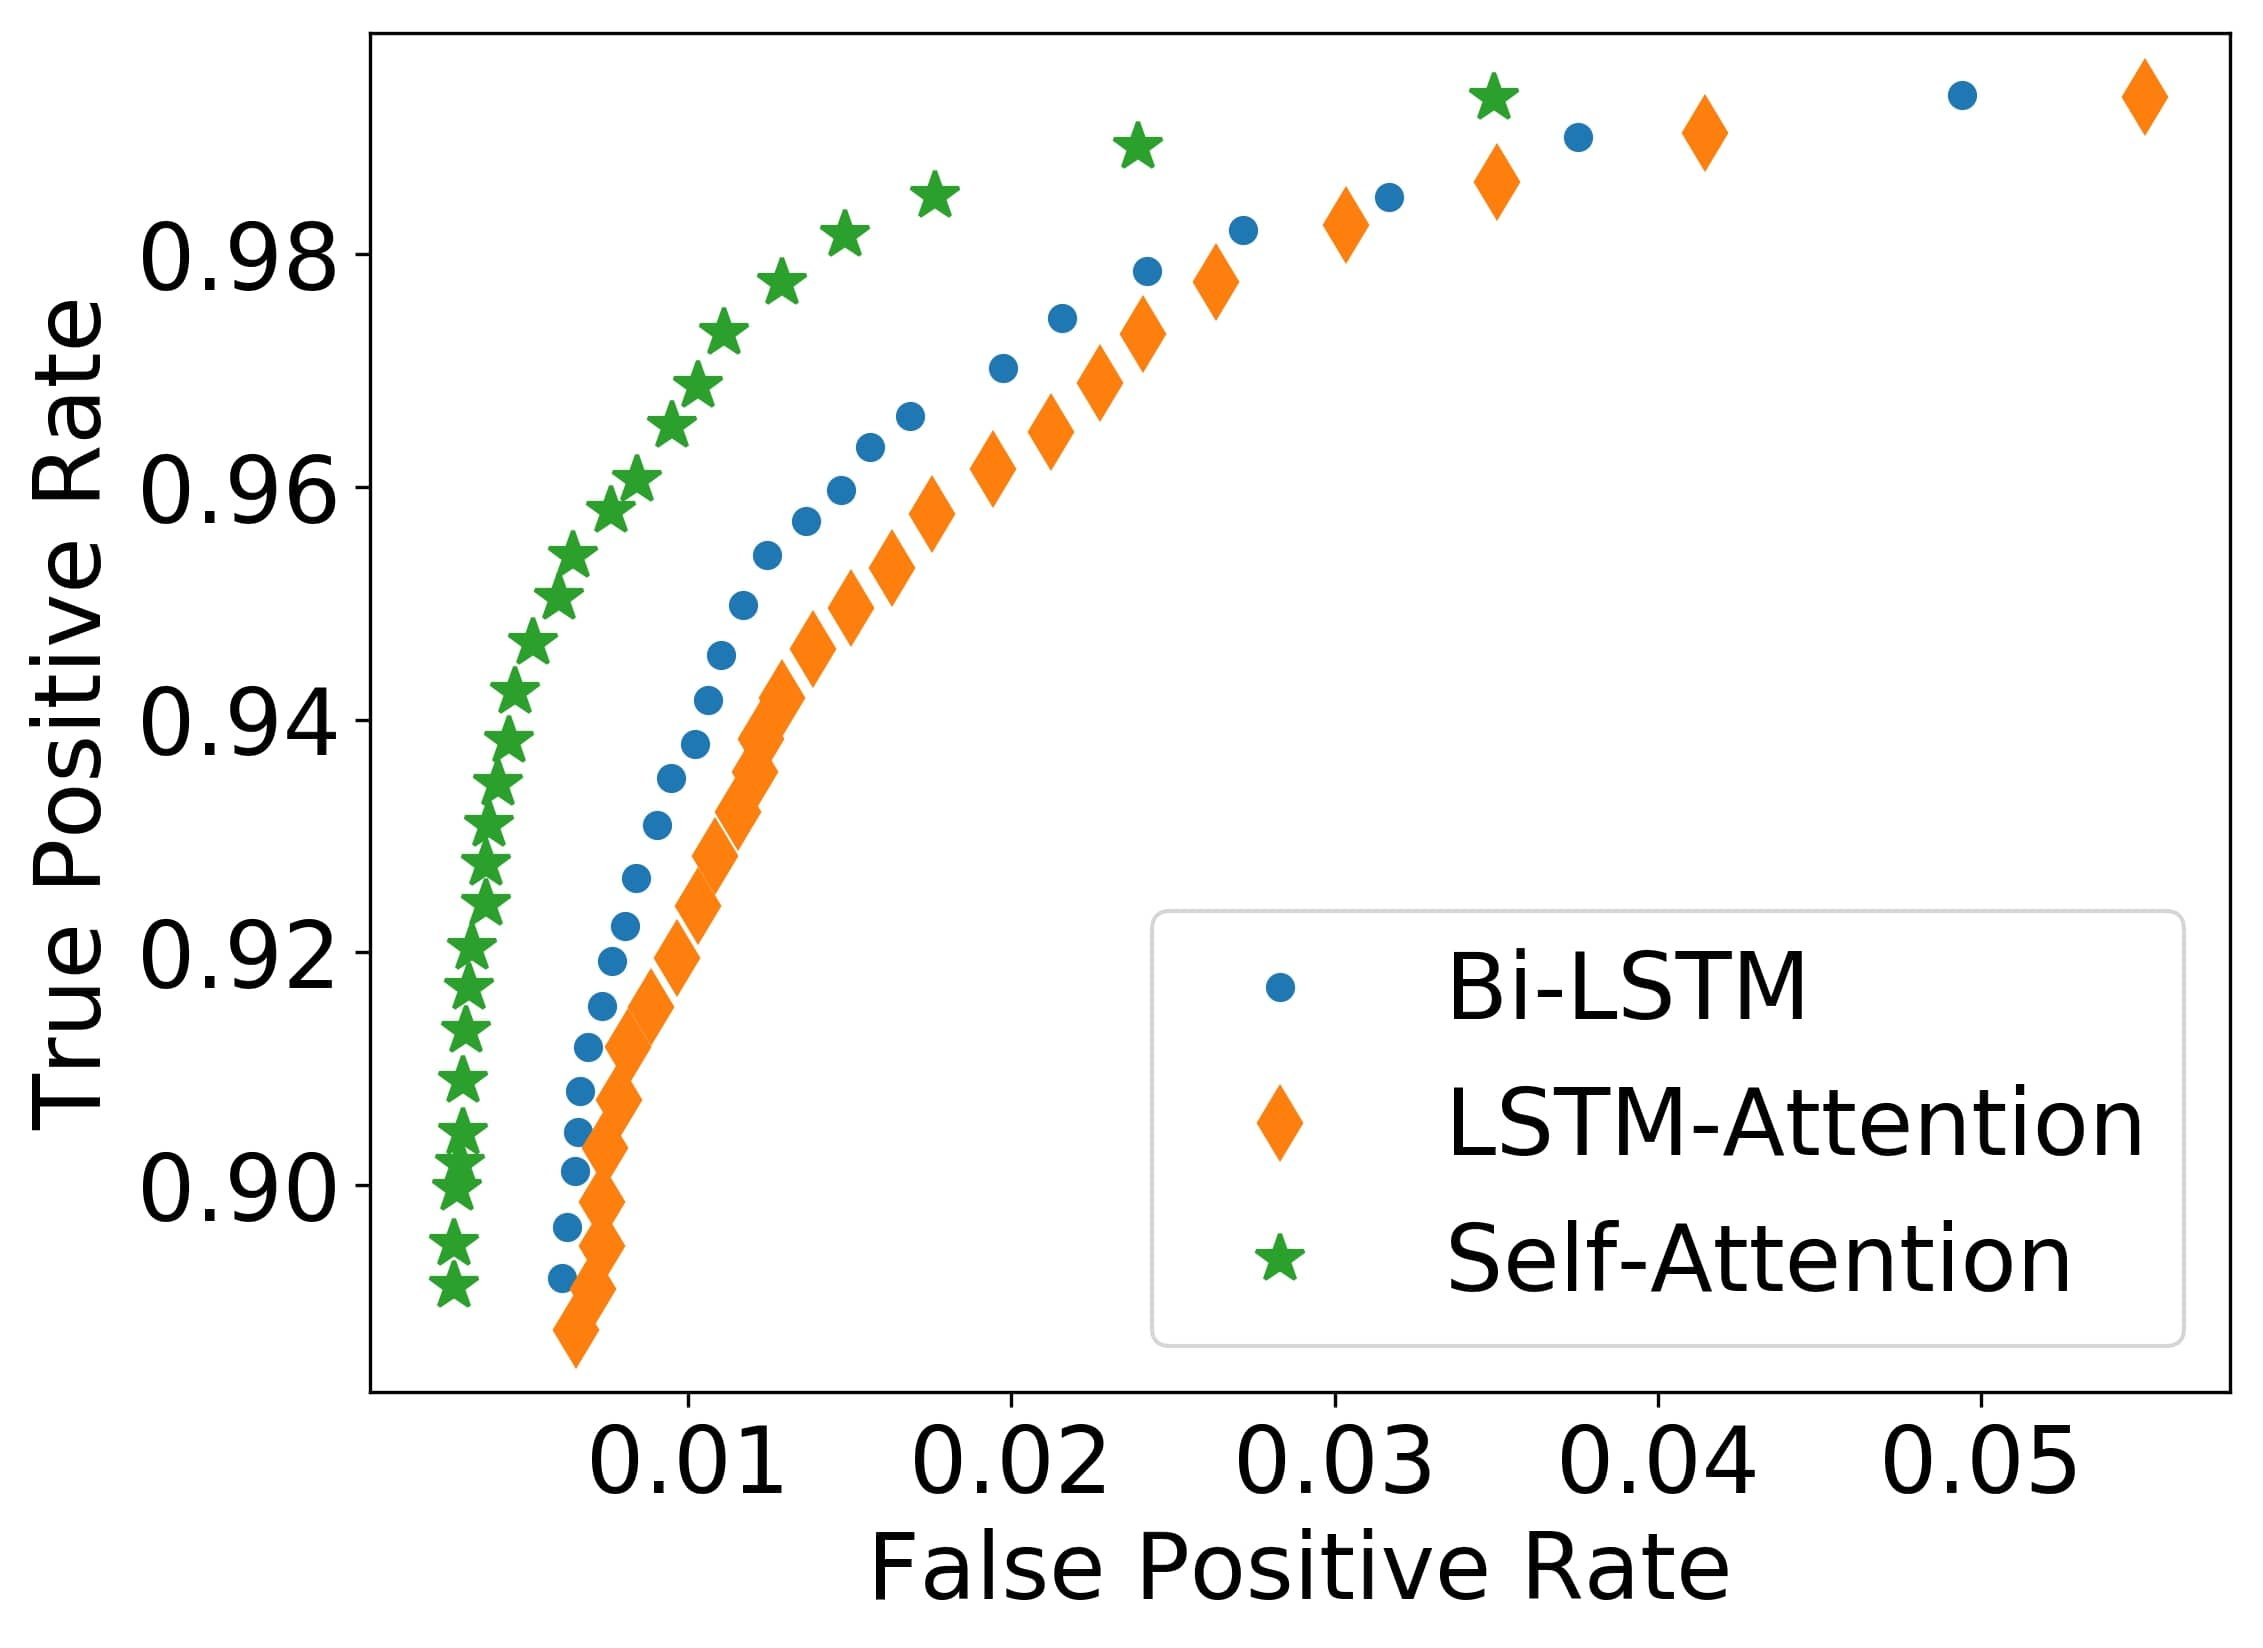}
\caption{DataRepo1}
\end{subfigure}
\begin{subfigure}{0.32\linewidth}
\includegraphics[width=0.85\linewidth]{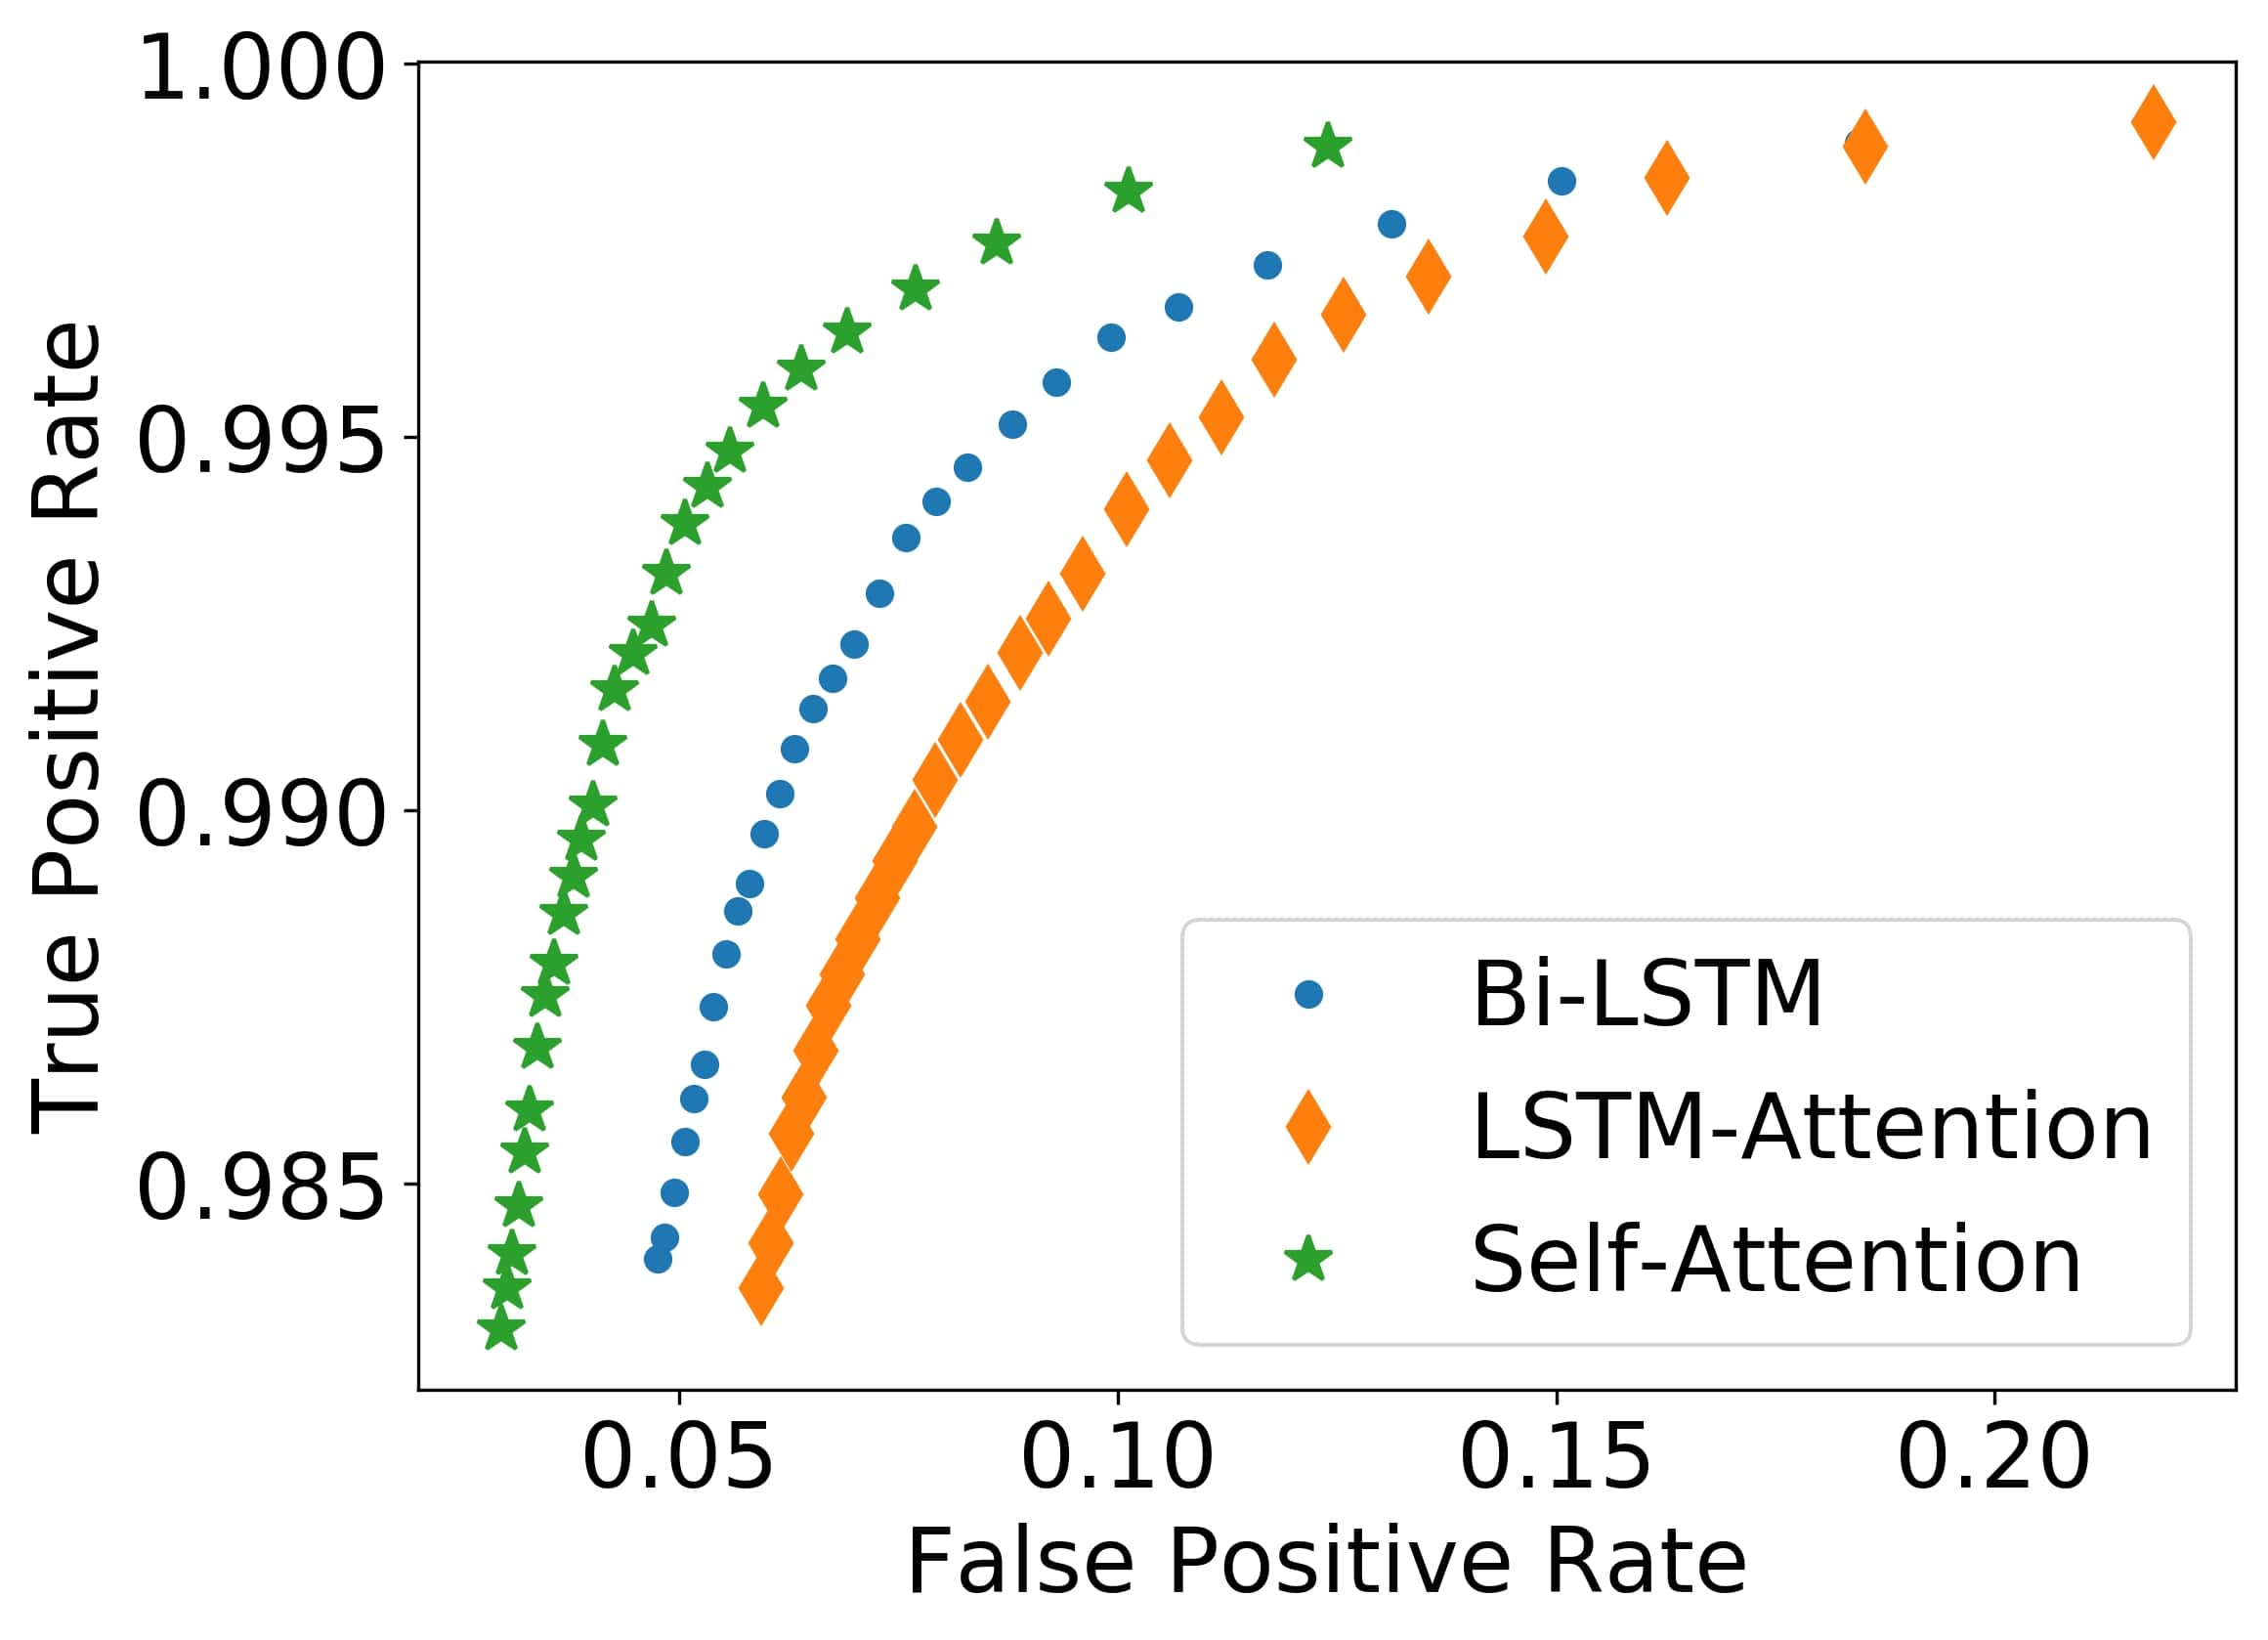}
\caption{DevOpsApp}
\end{subfigure}
\begin{subfigure}{0.32\linewidth}
\includegraphics[width=0.85\linewidth]{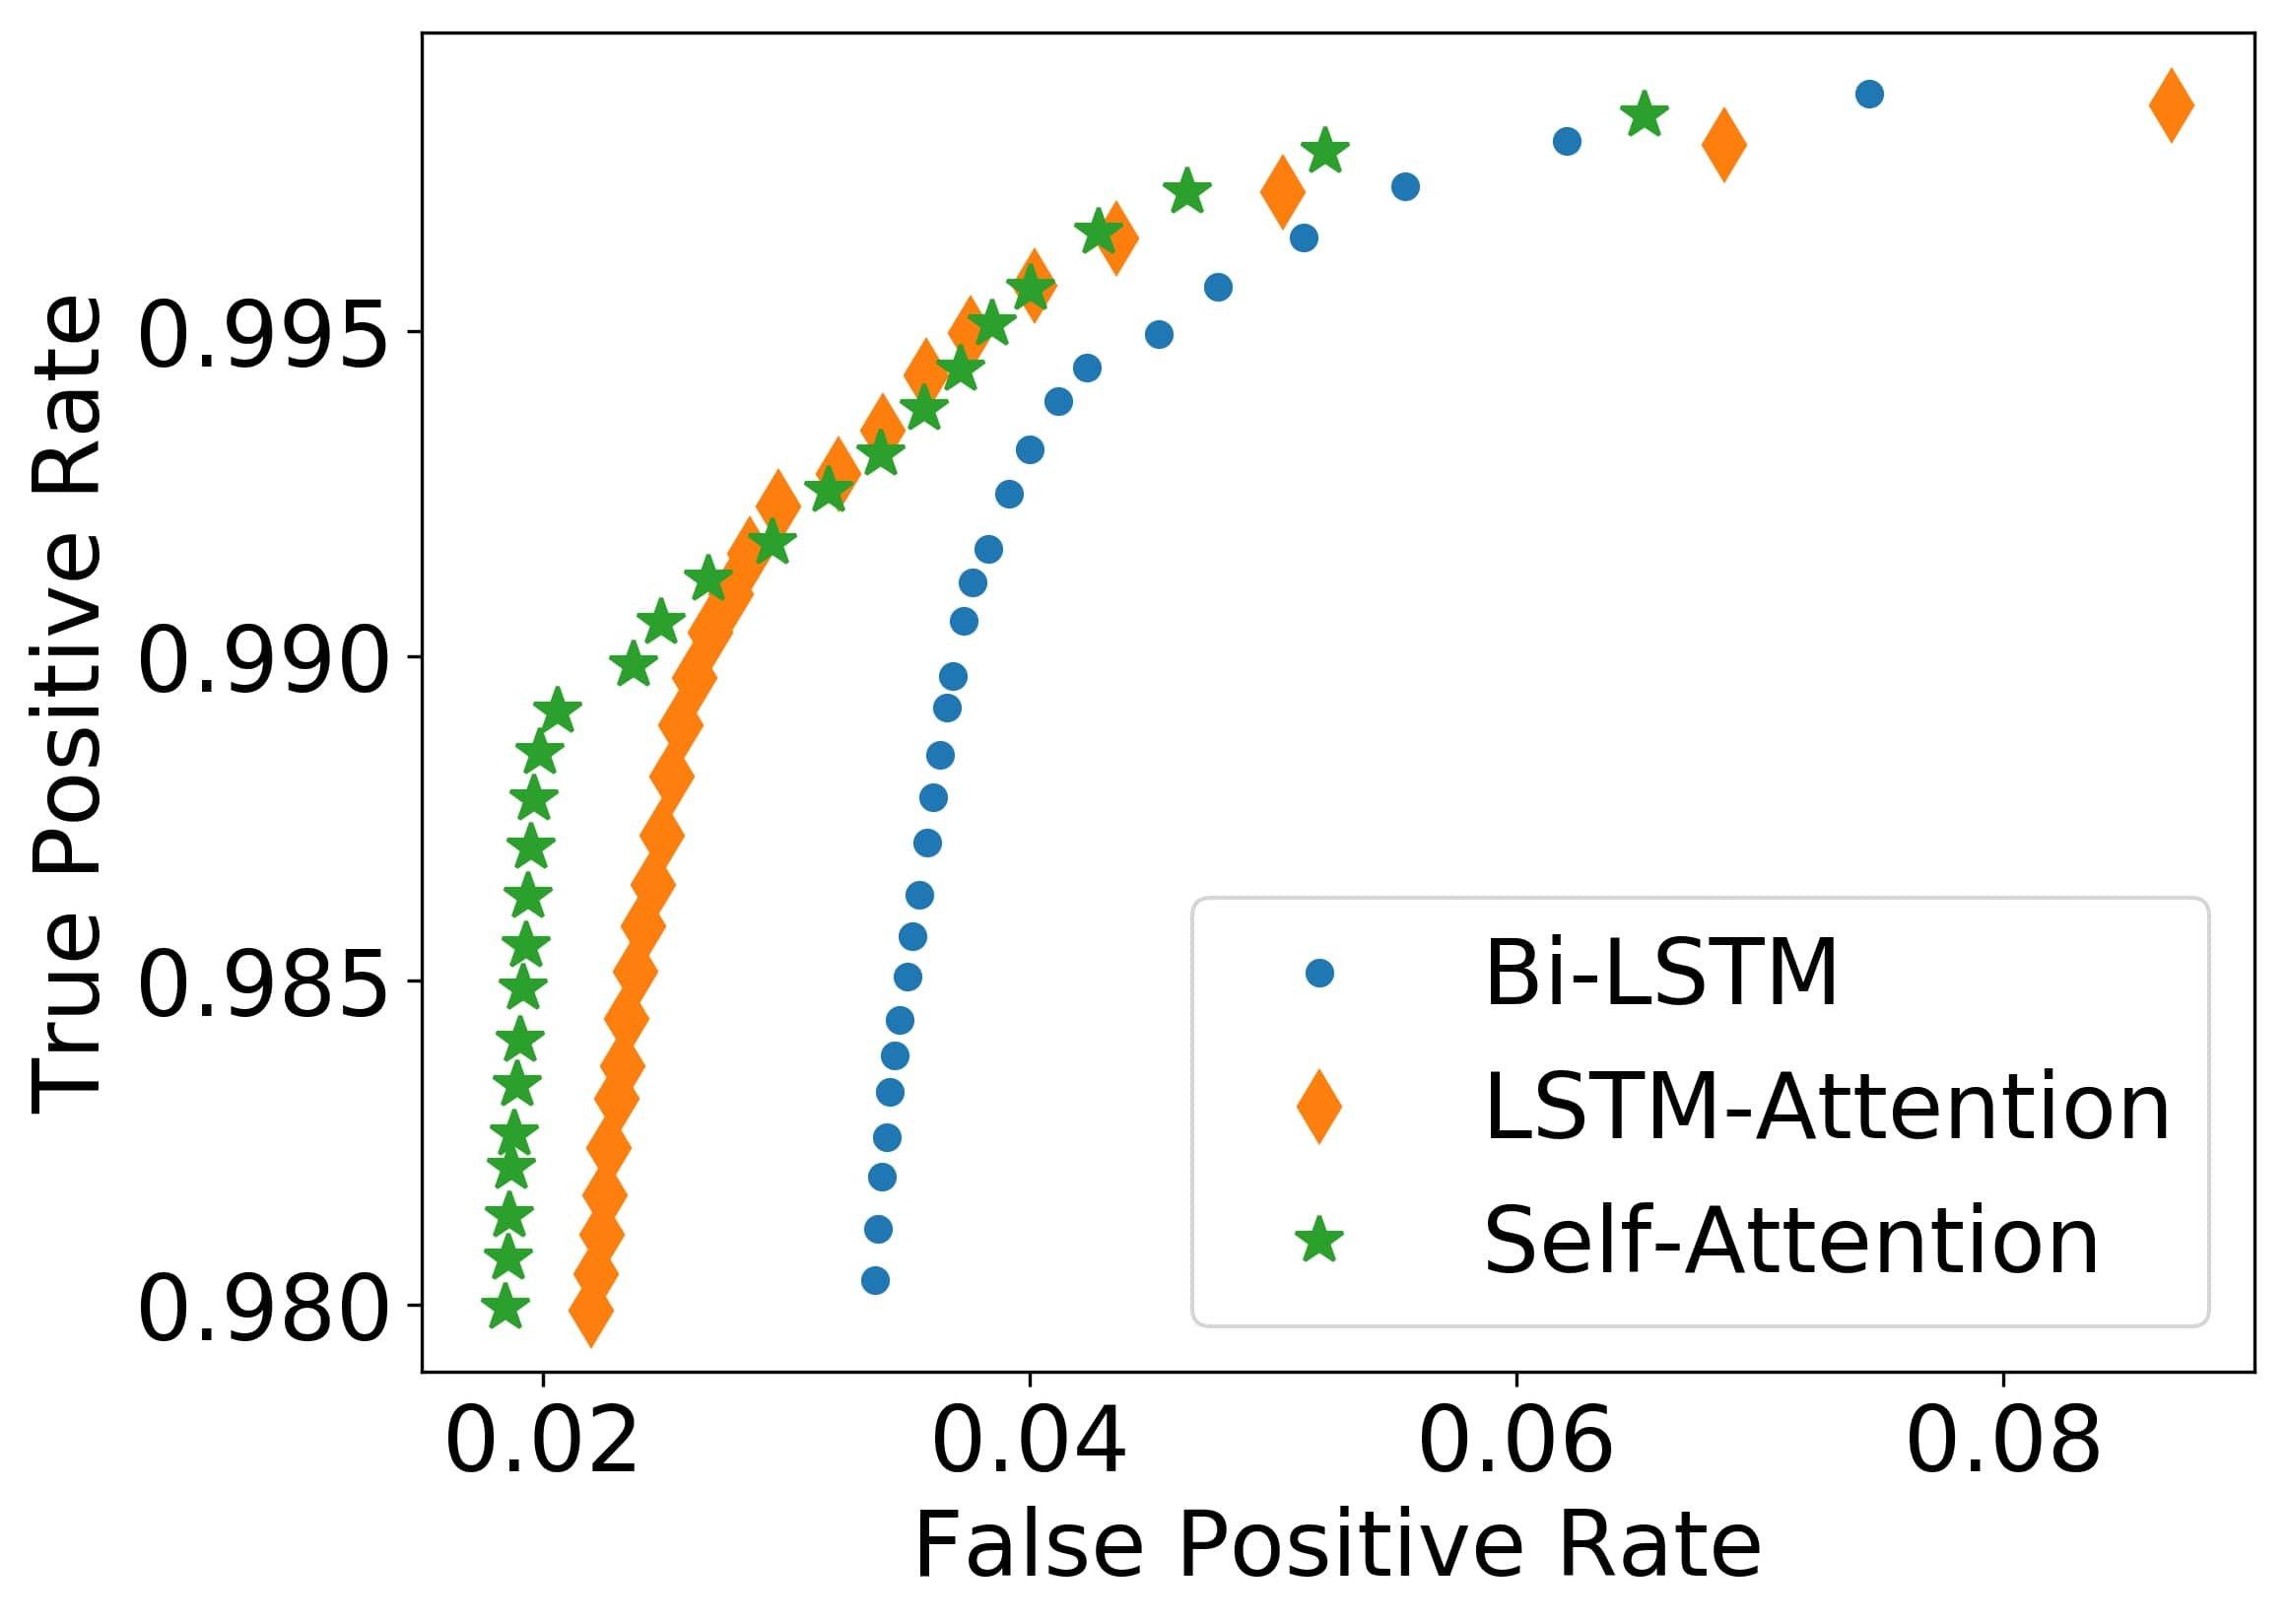}
\caption{DataAnalyzer1}
\end{subfigure}
\begin{subfigure}{0.32\linewidth}
\includegraphics[width=0.85\linewidth]{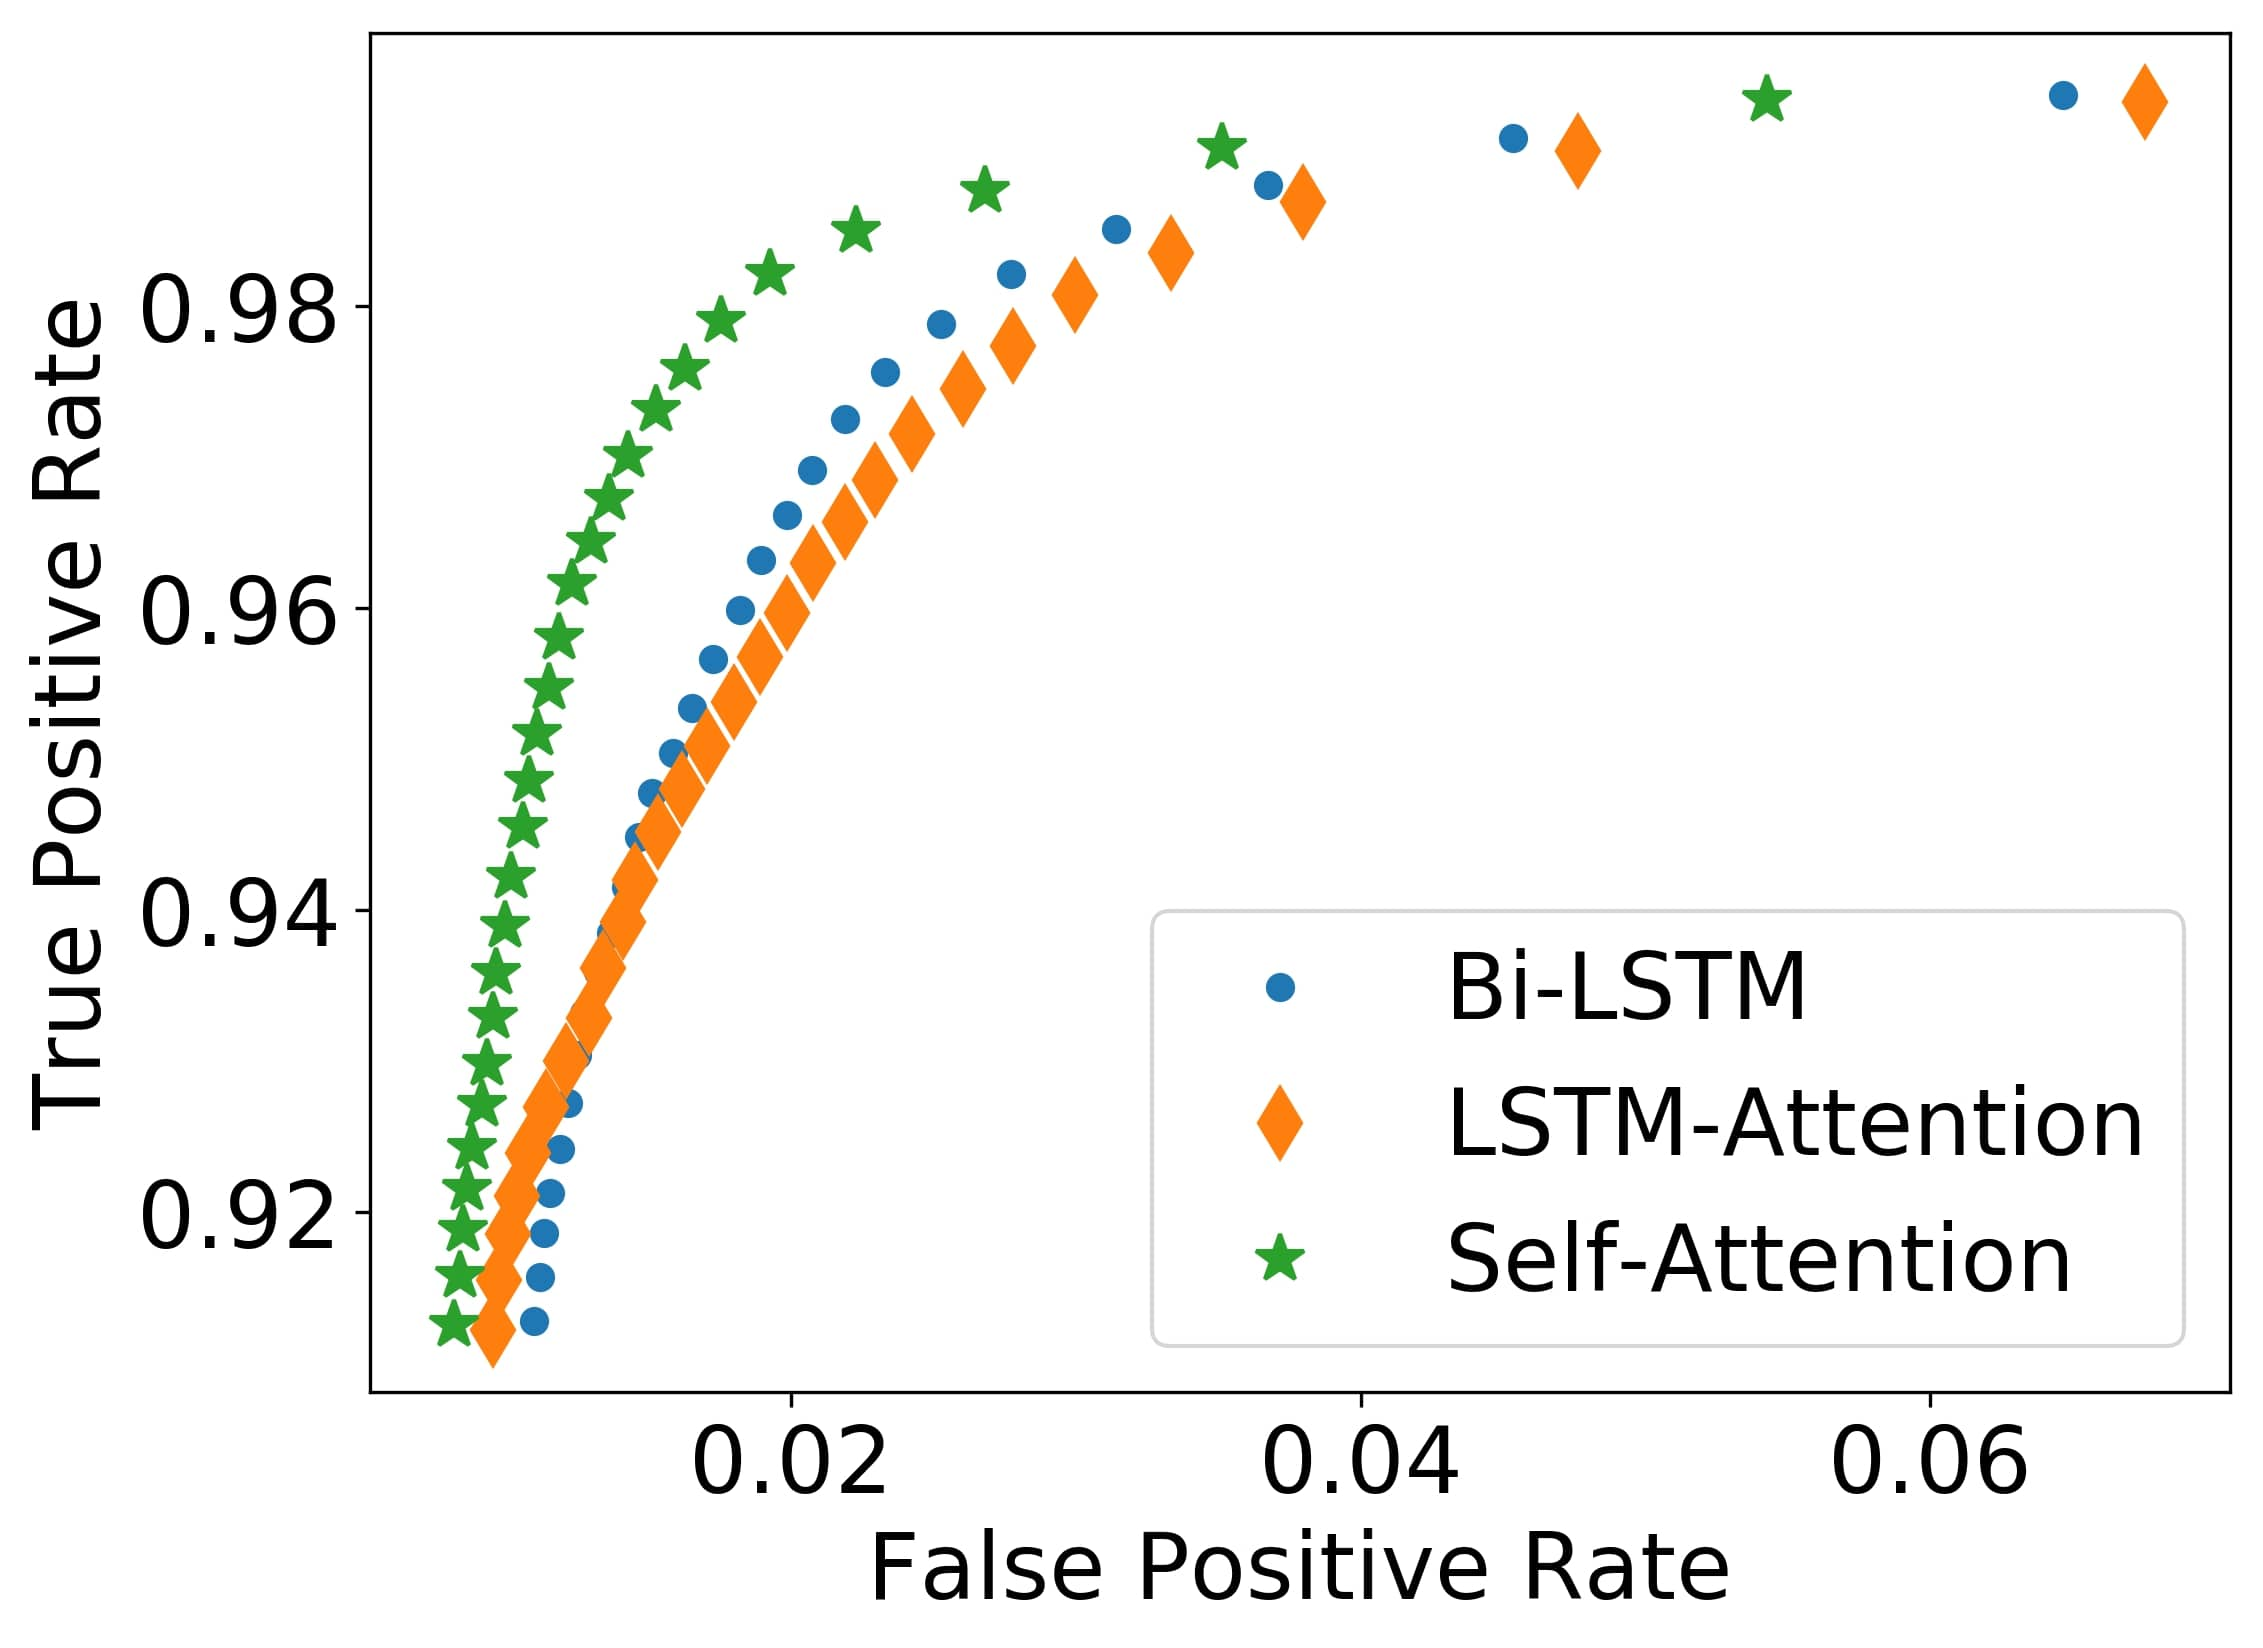}
\caption{DataAnalyzer2}
\end{subfigure}
\begin{subfigure}{0.32\linewidth}
\includegraphics[width=0.85\linewidth]{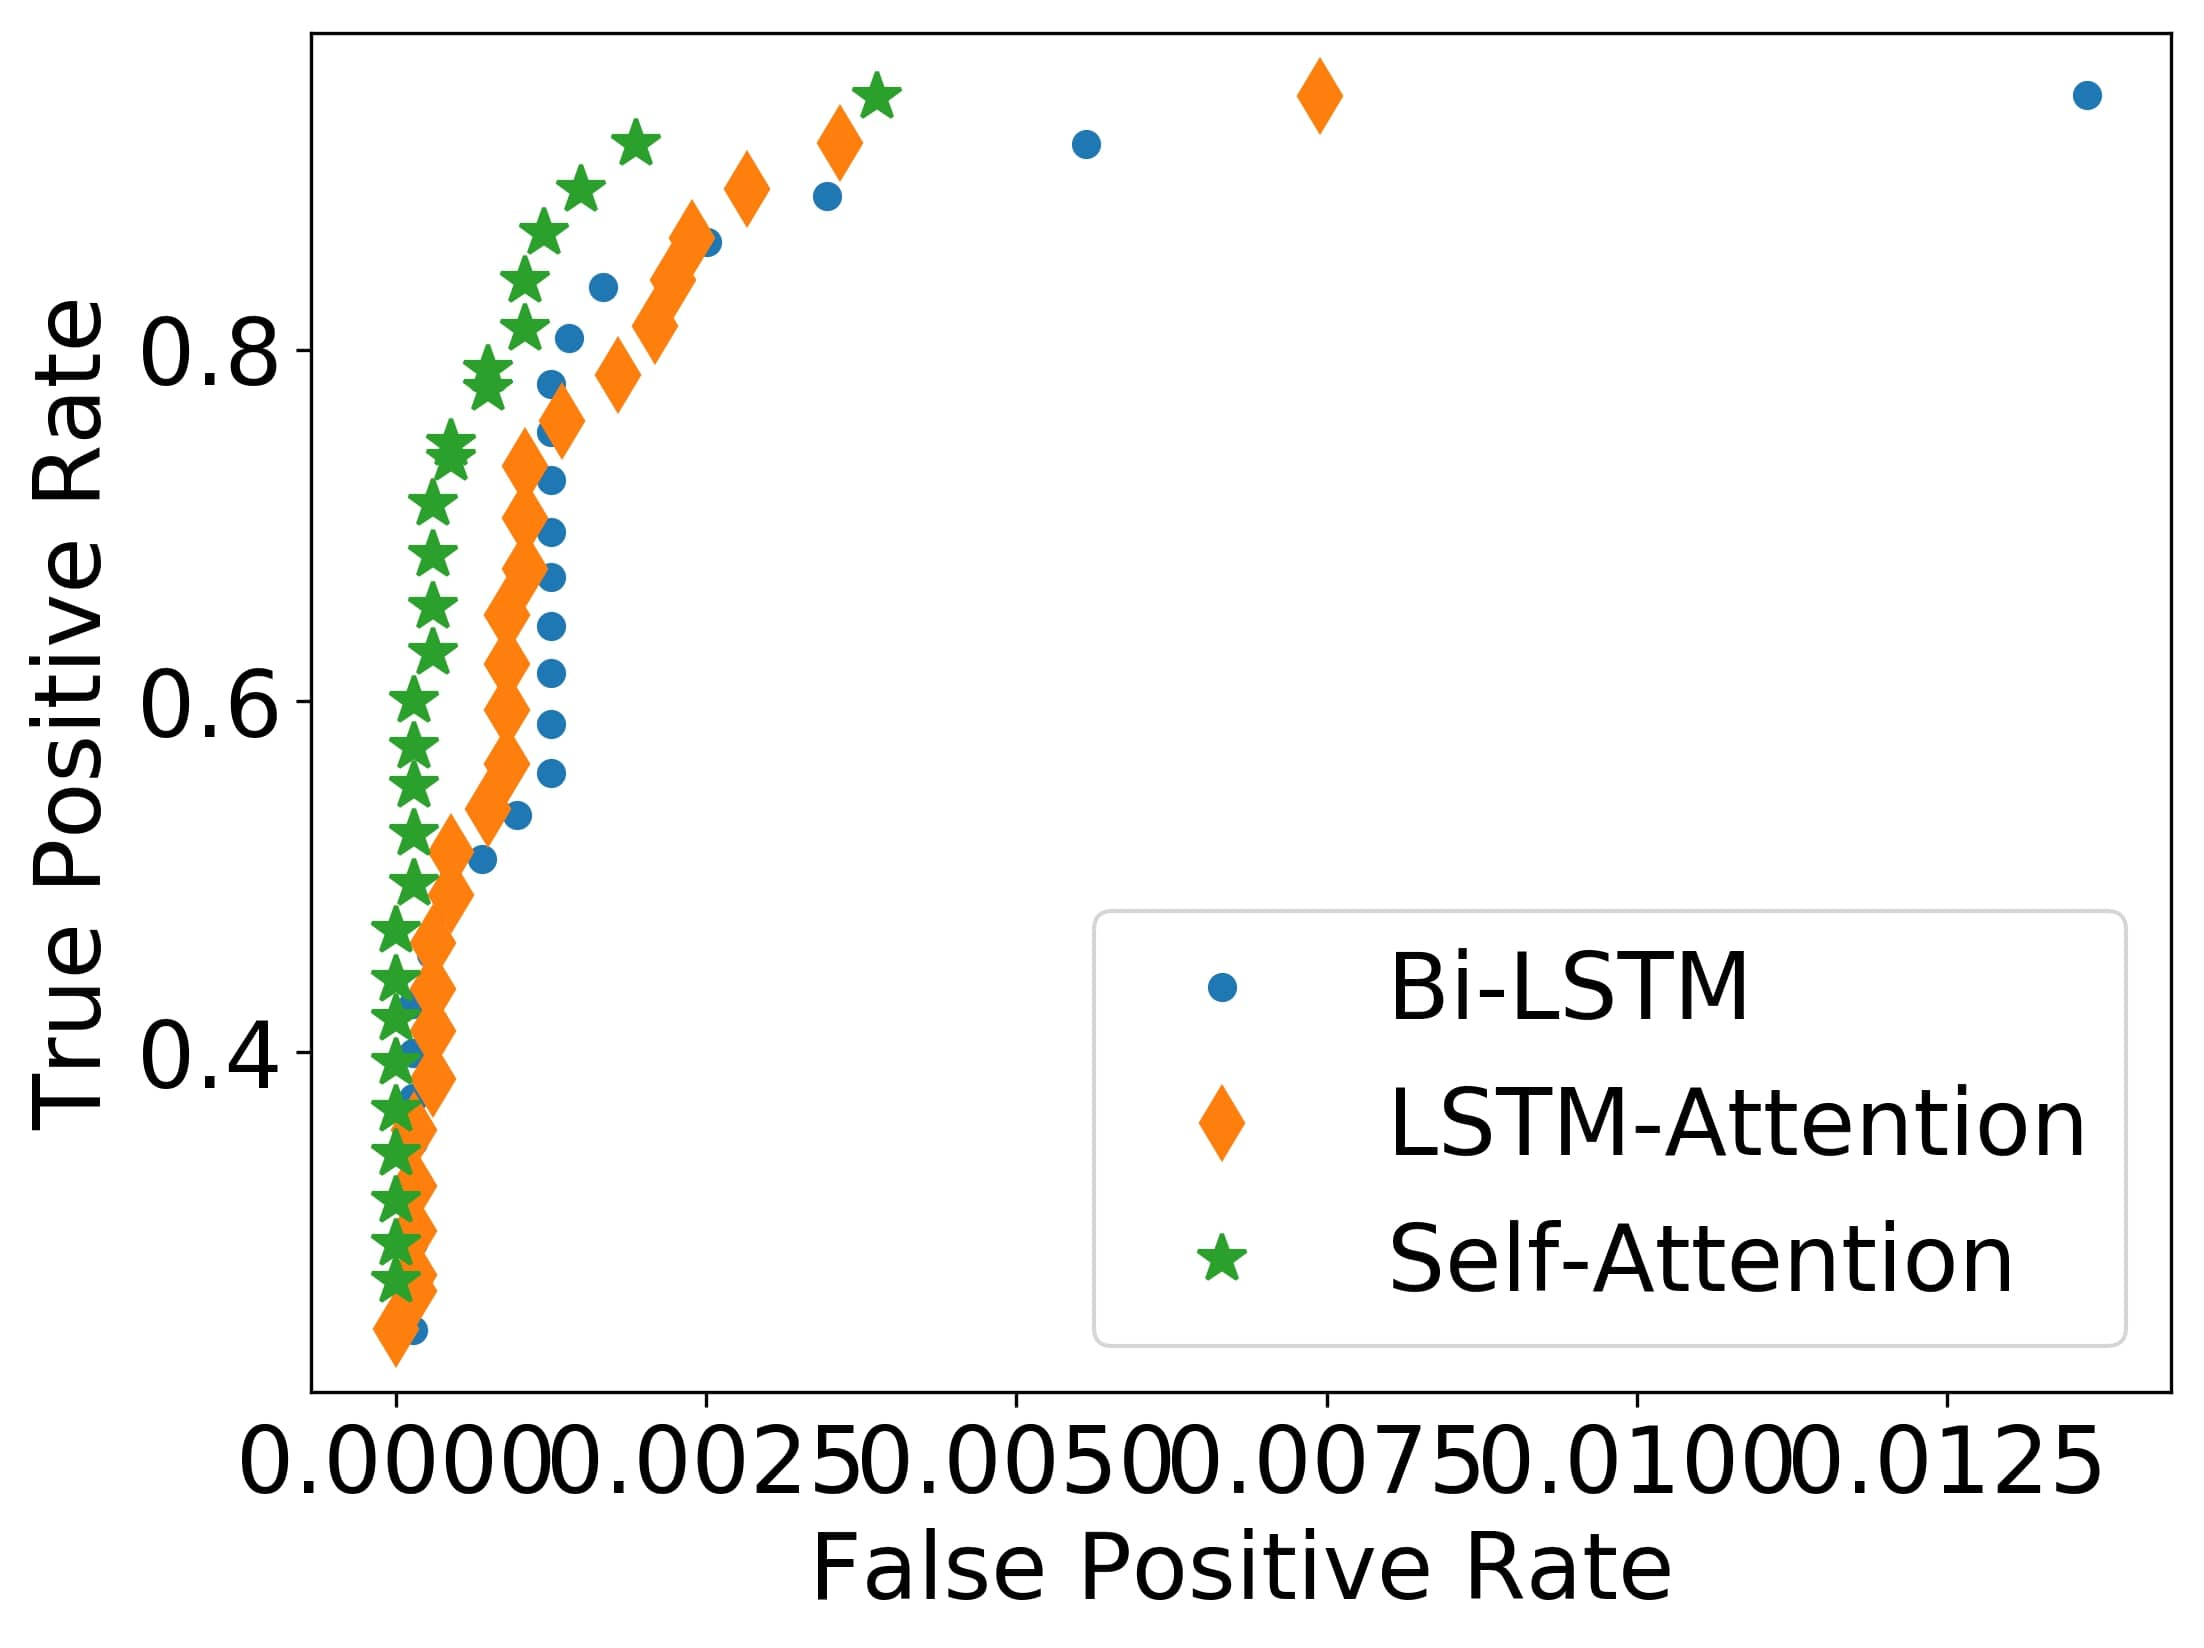}
\caption{DataRepo2}
\end{subfigure}
\caption{ROC Curve Comparison (Predicting Centered Events).}
\label{fig:roc_offline}
\end{figure*}

\begin{figure*}[!tb]
\centering
\begin{subfigure}{0.32\linewidth}
\centering
\includegraphics[width=0.85\linewidth]{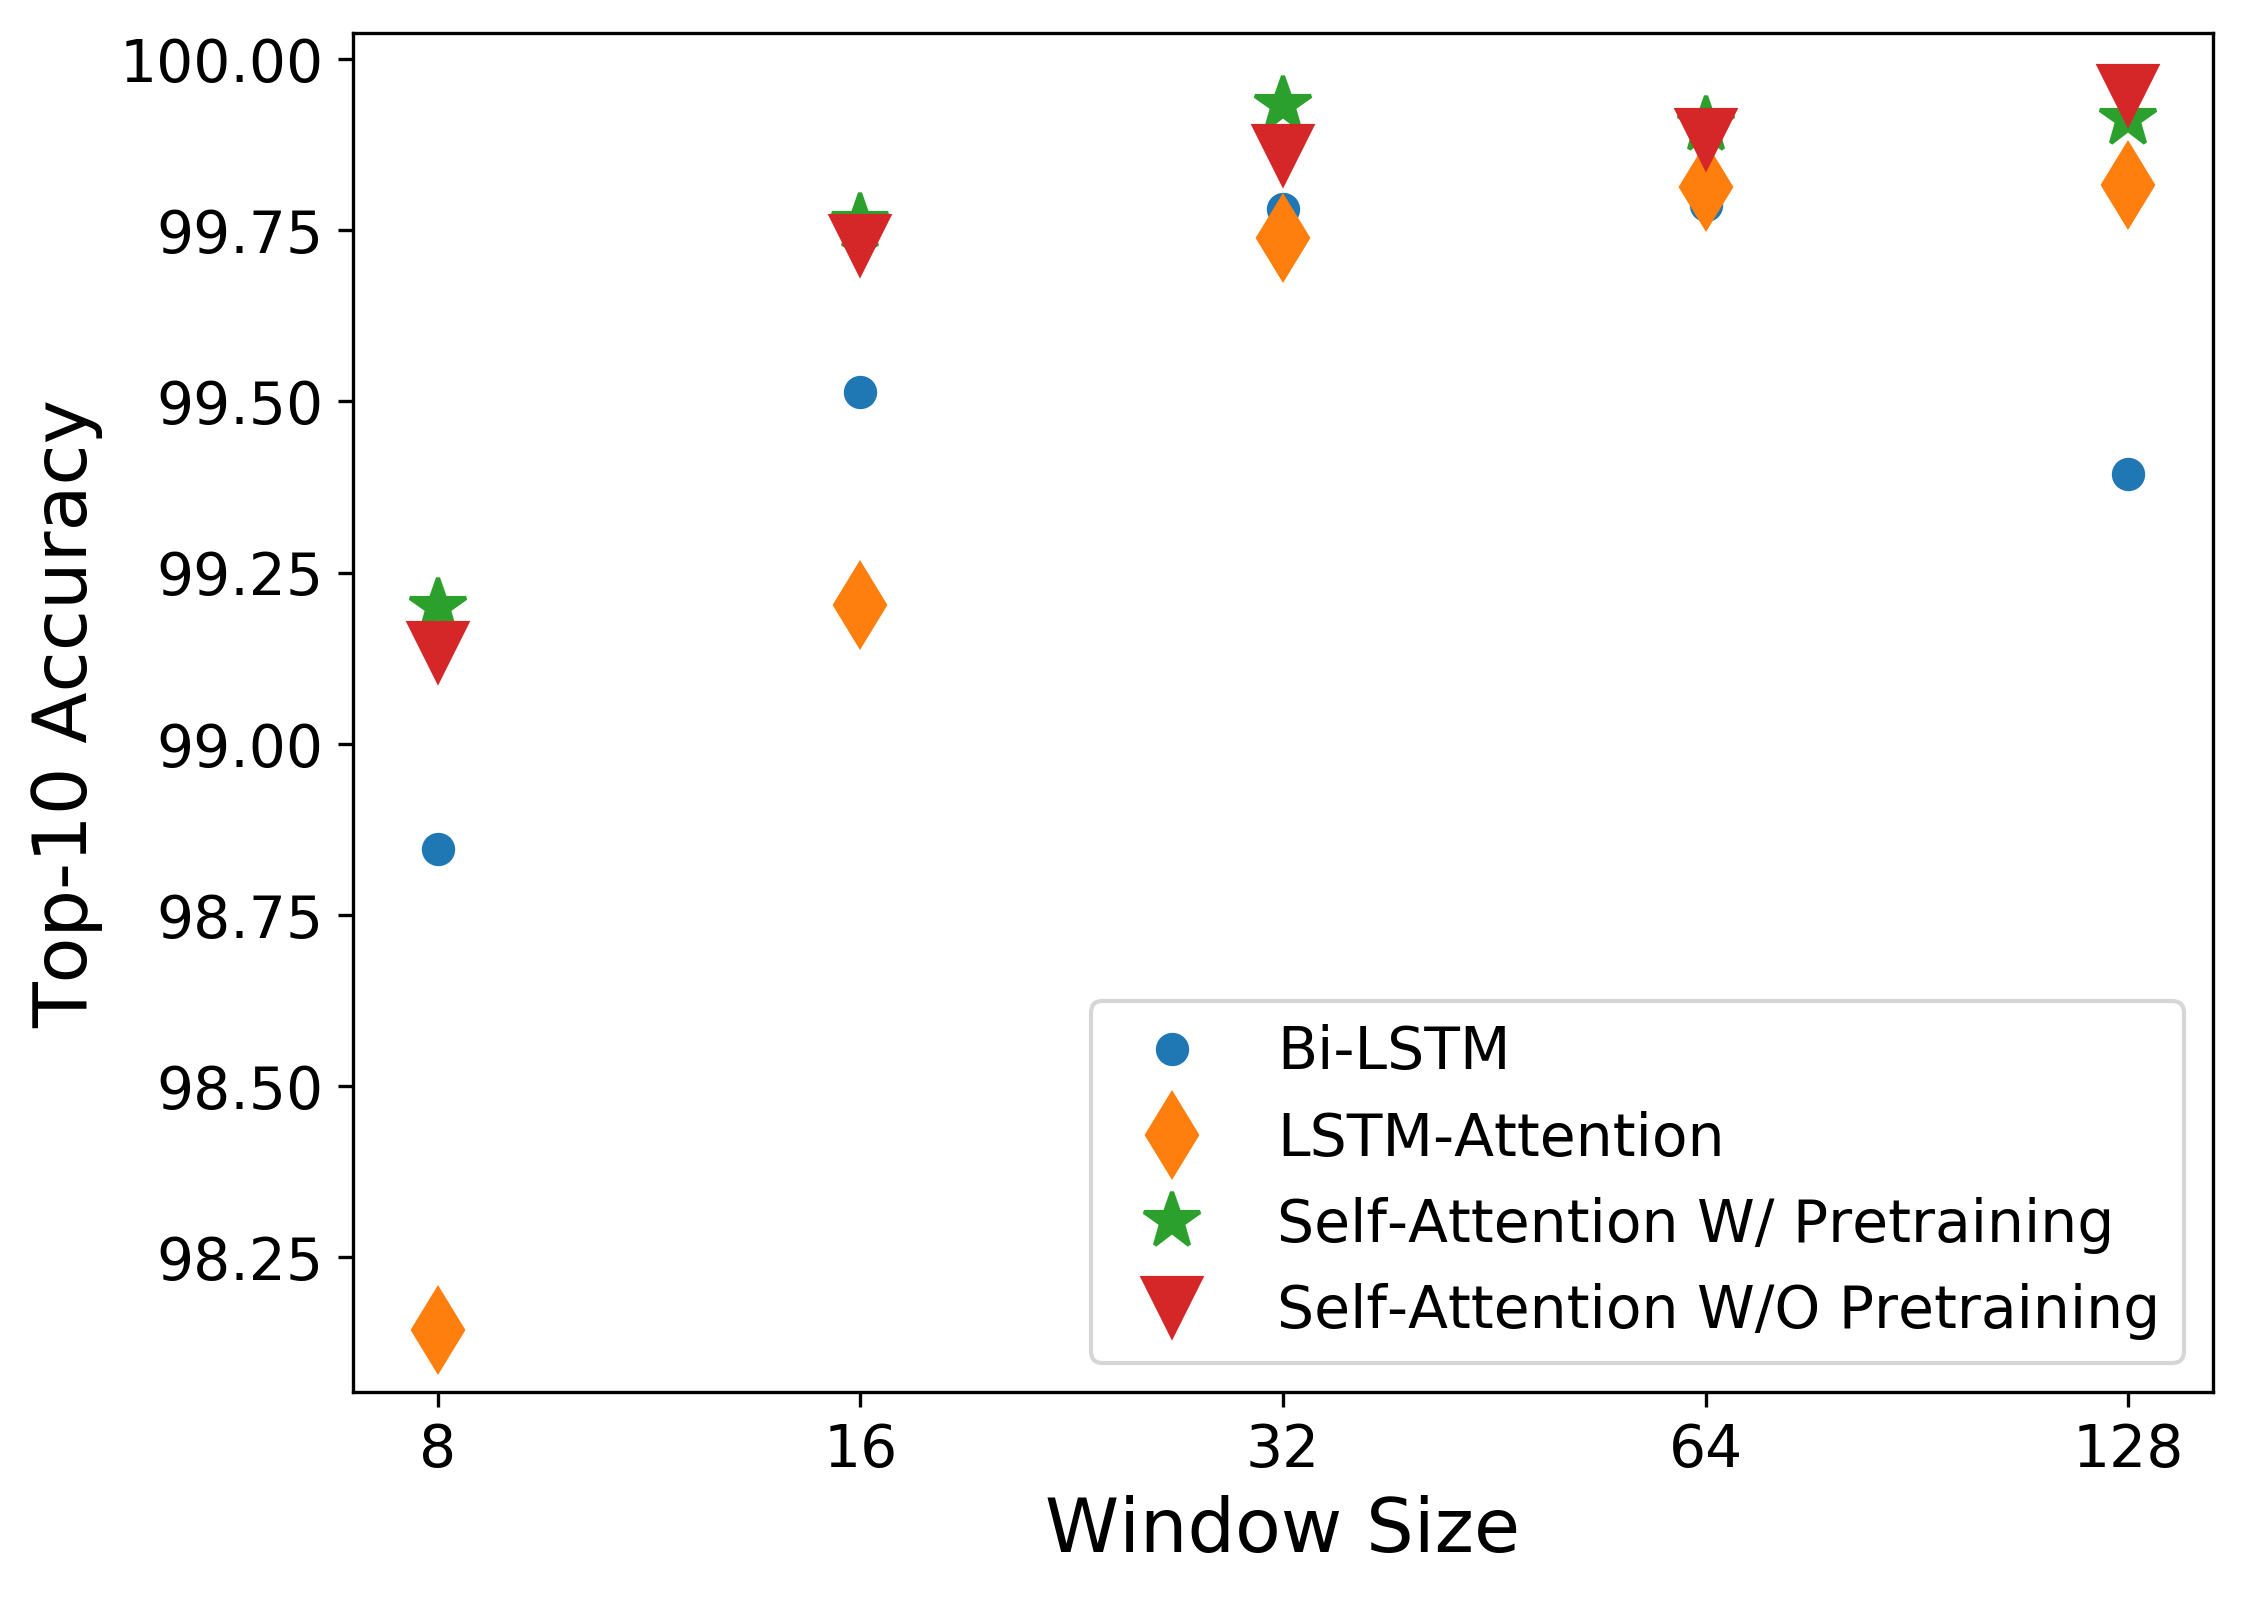}
\caption{Workqueue}
\end{subfigure}
\begin{subfigure}{0.32\linewidth}
\centering
\includegraphics[width=0.85\linewidth]{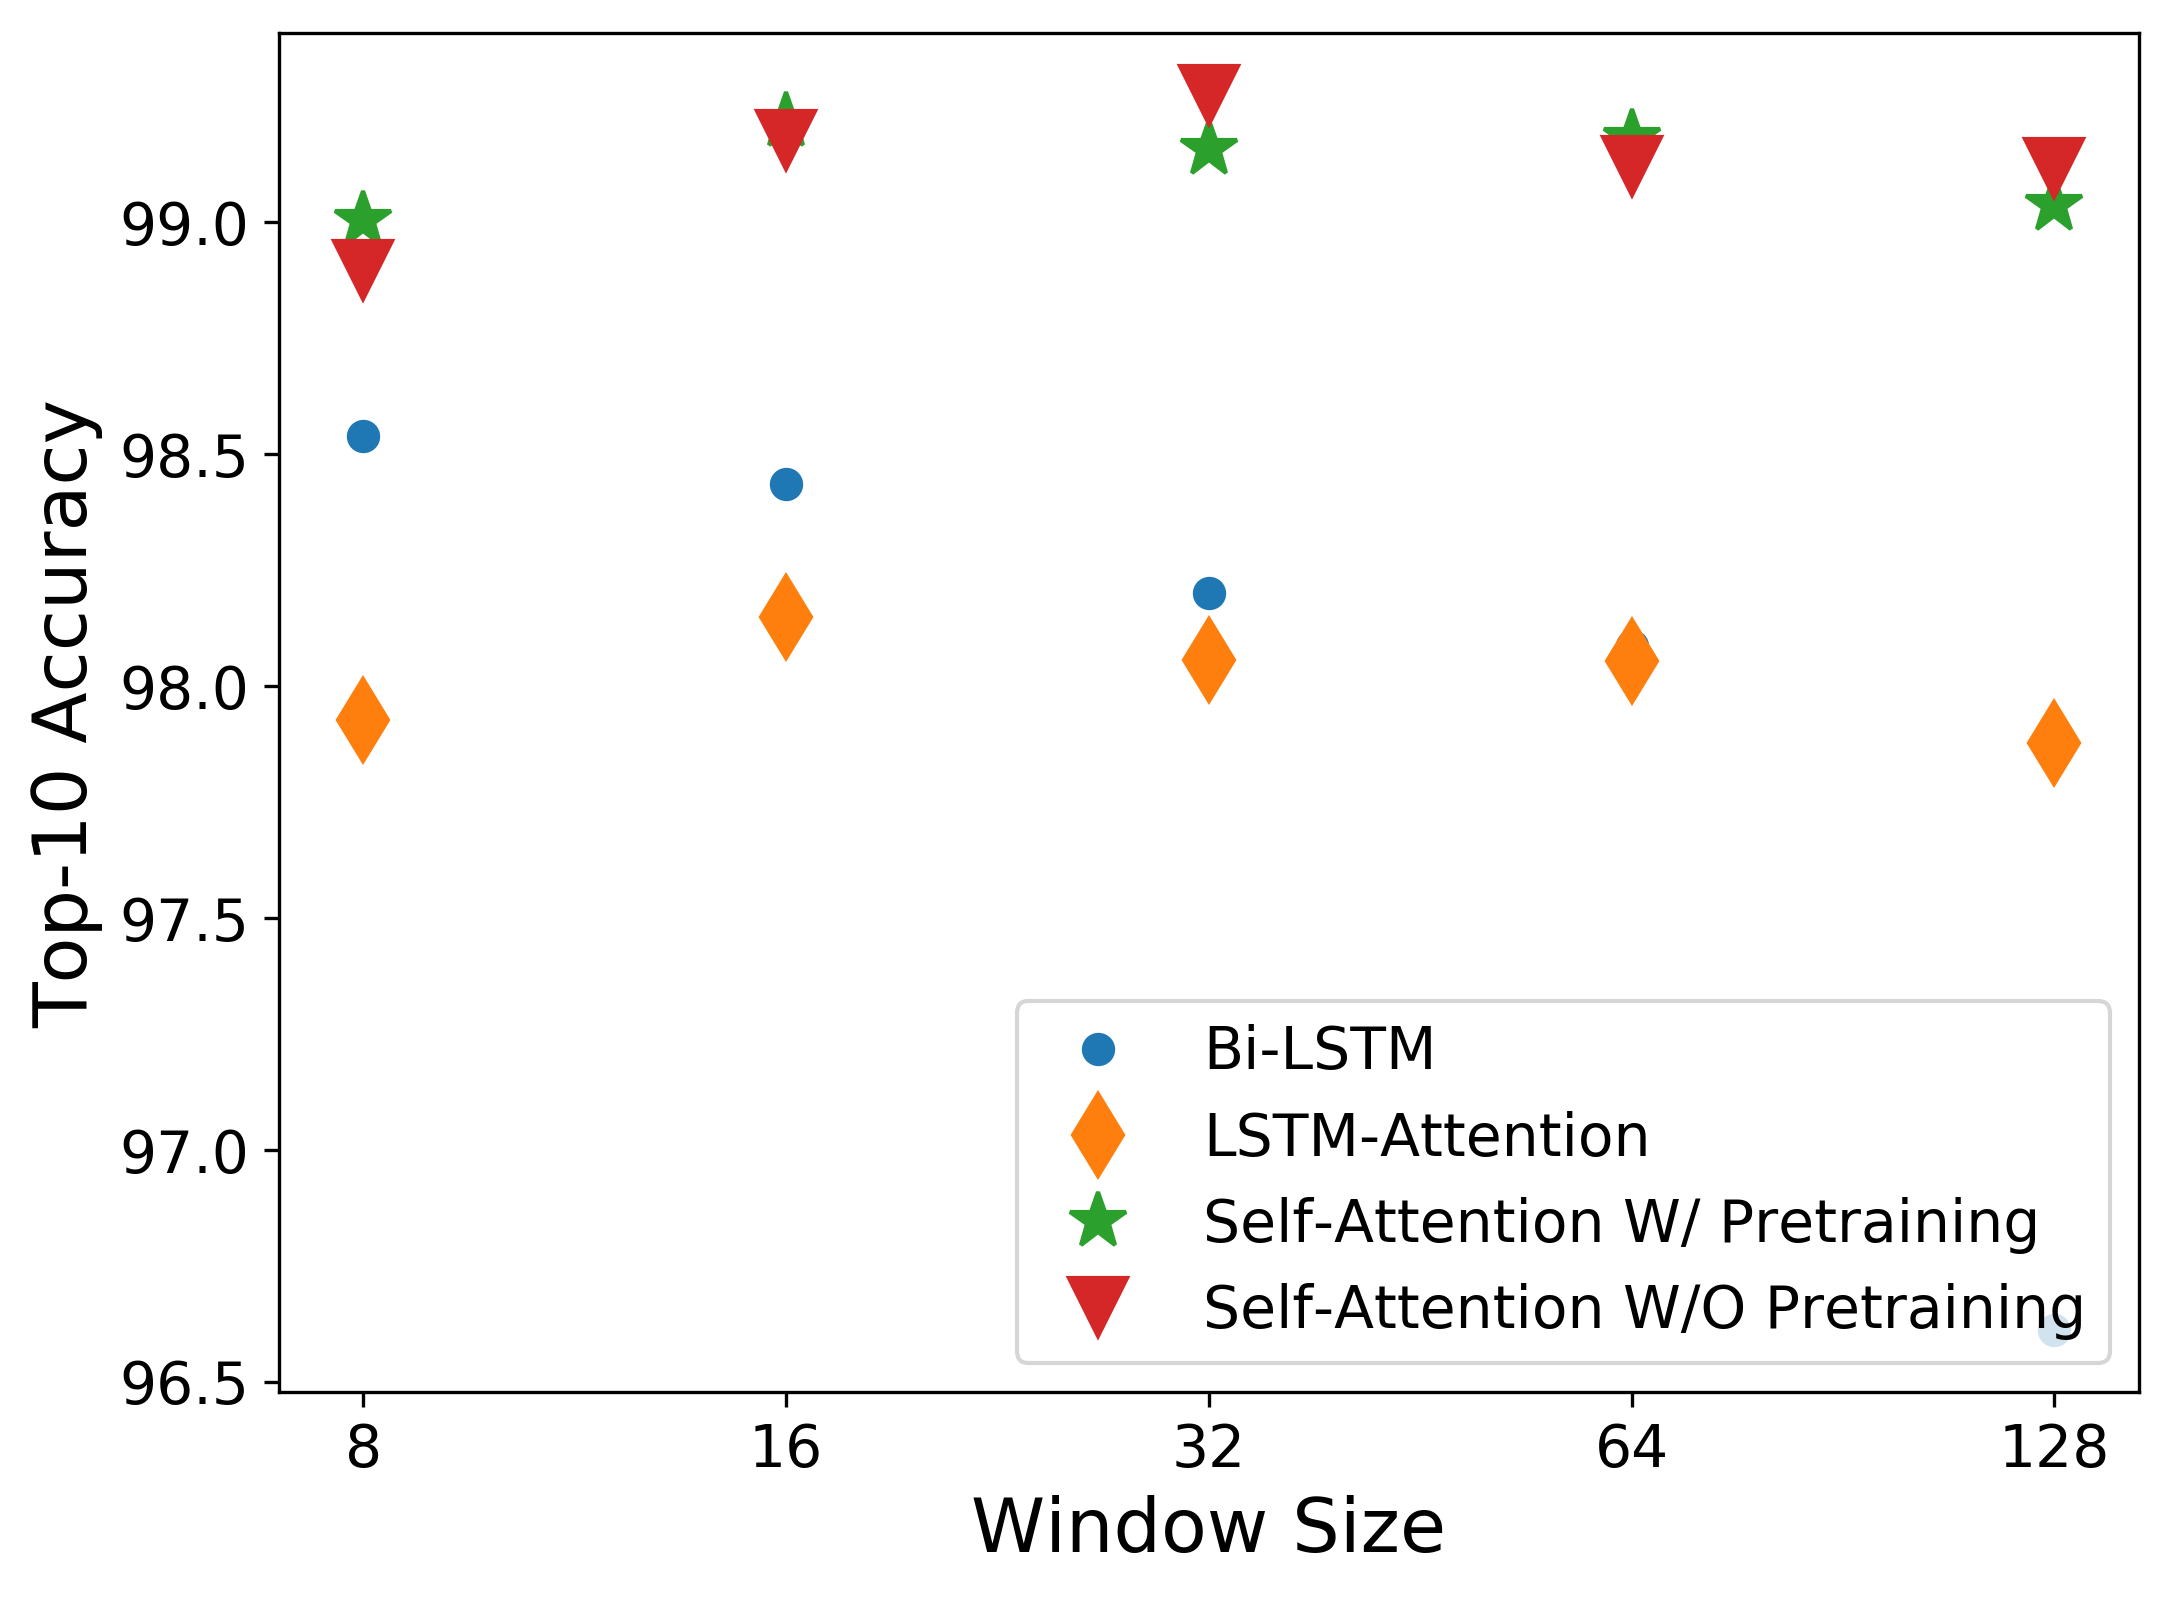}
\caption{DataRepo1}
\end{subfigure}
\begin{subfigure}{0.32\linewidth}
\centering
\includegraphics[width=0.85\linewidth]{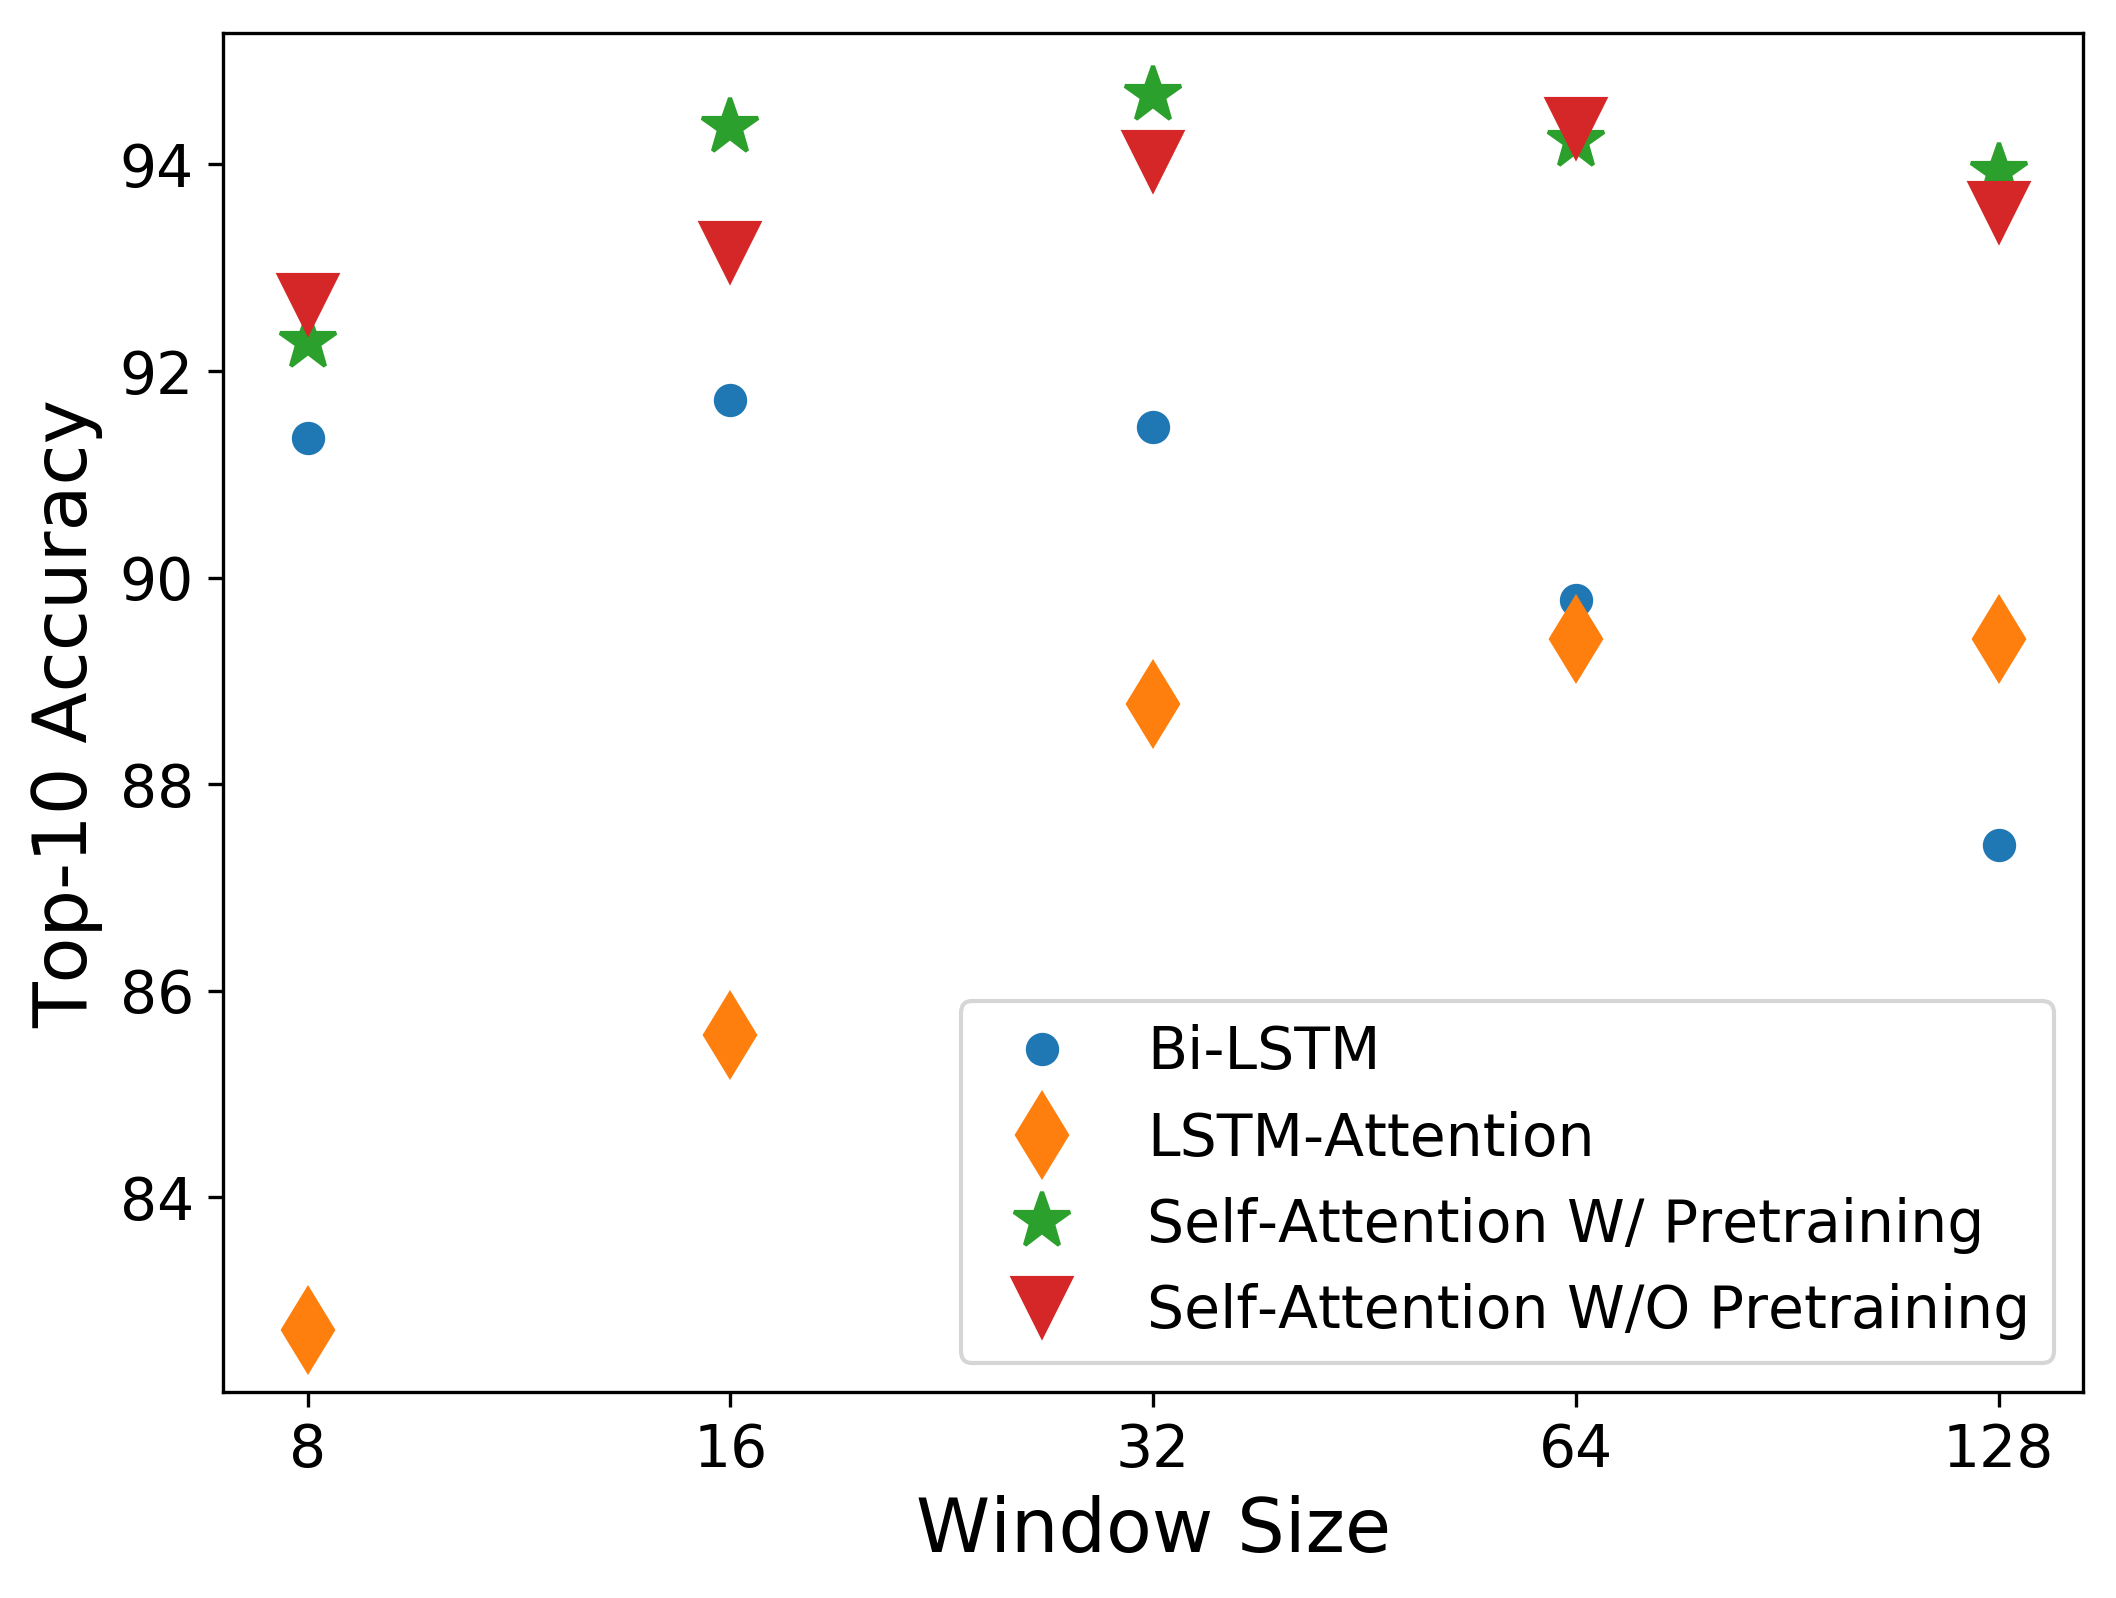}
\caption{DevOpsApp}
\end{subfigure}
\begin{subfigure}{0.32\linewidth}
\centering
\includegraphics[width=0.85\linewidth]{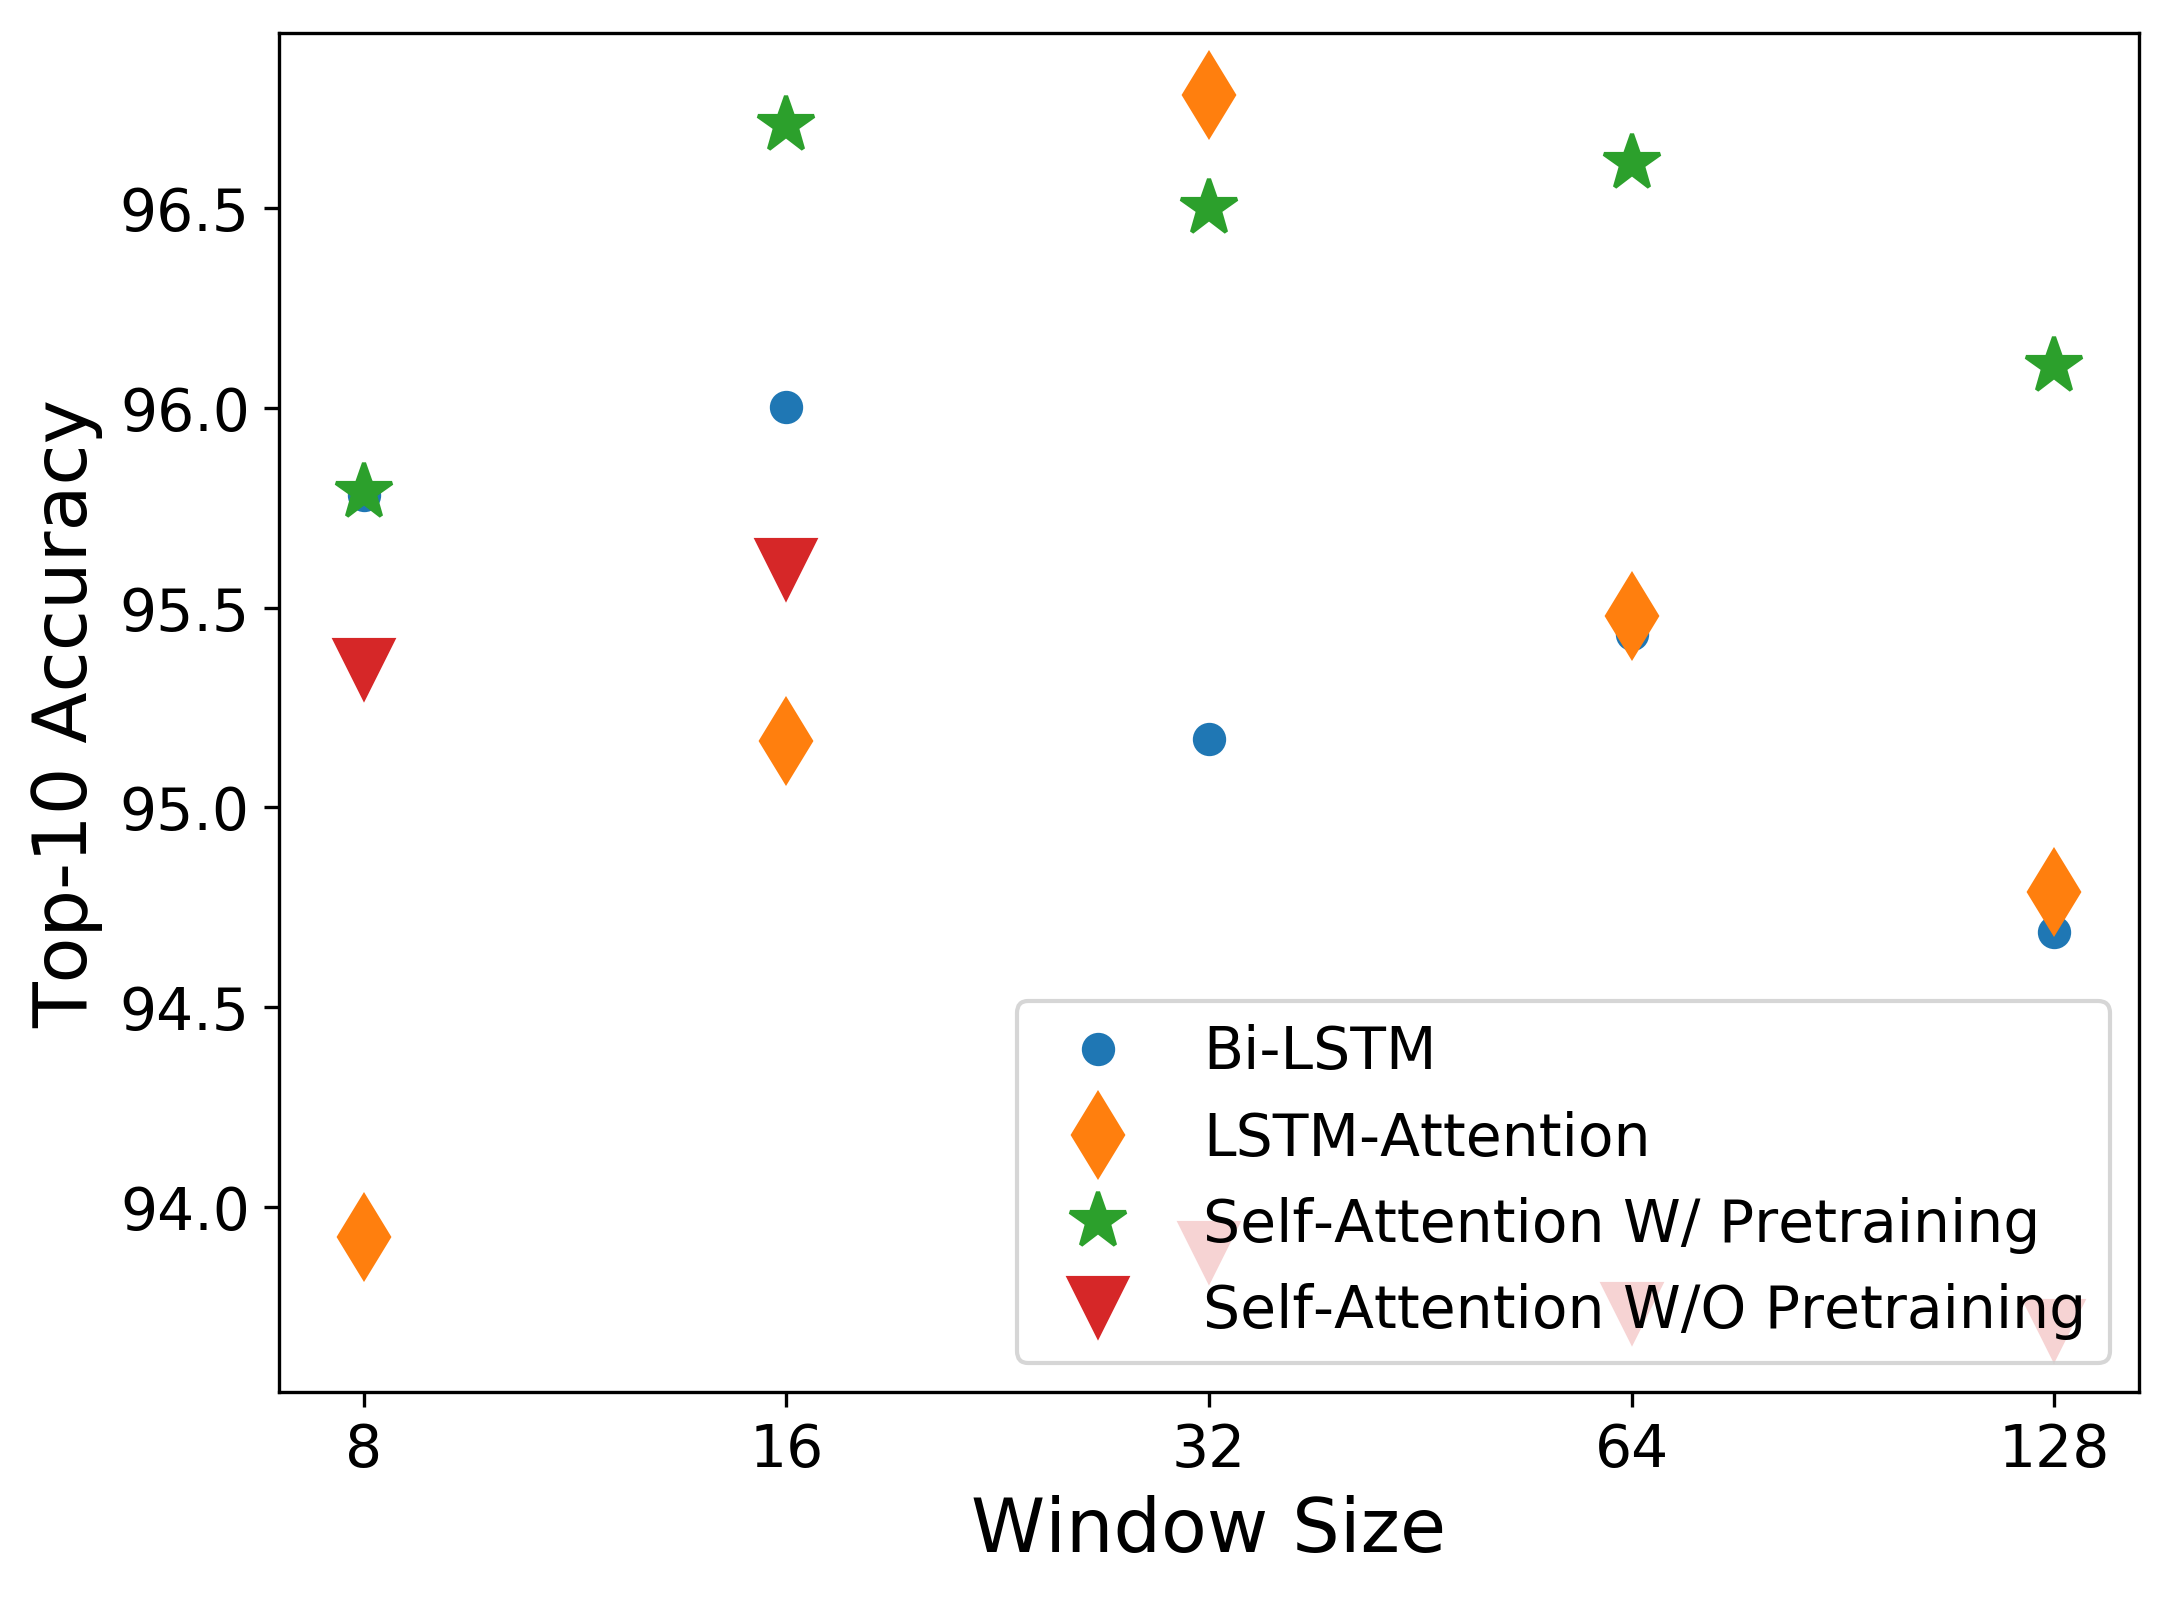}
\caption{DataAnalyzer1}
\end{subfigure}
\begin{subfigure}{0.32\linewidth}
\centering
\includegraphics[width=0.85\linewidth]{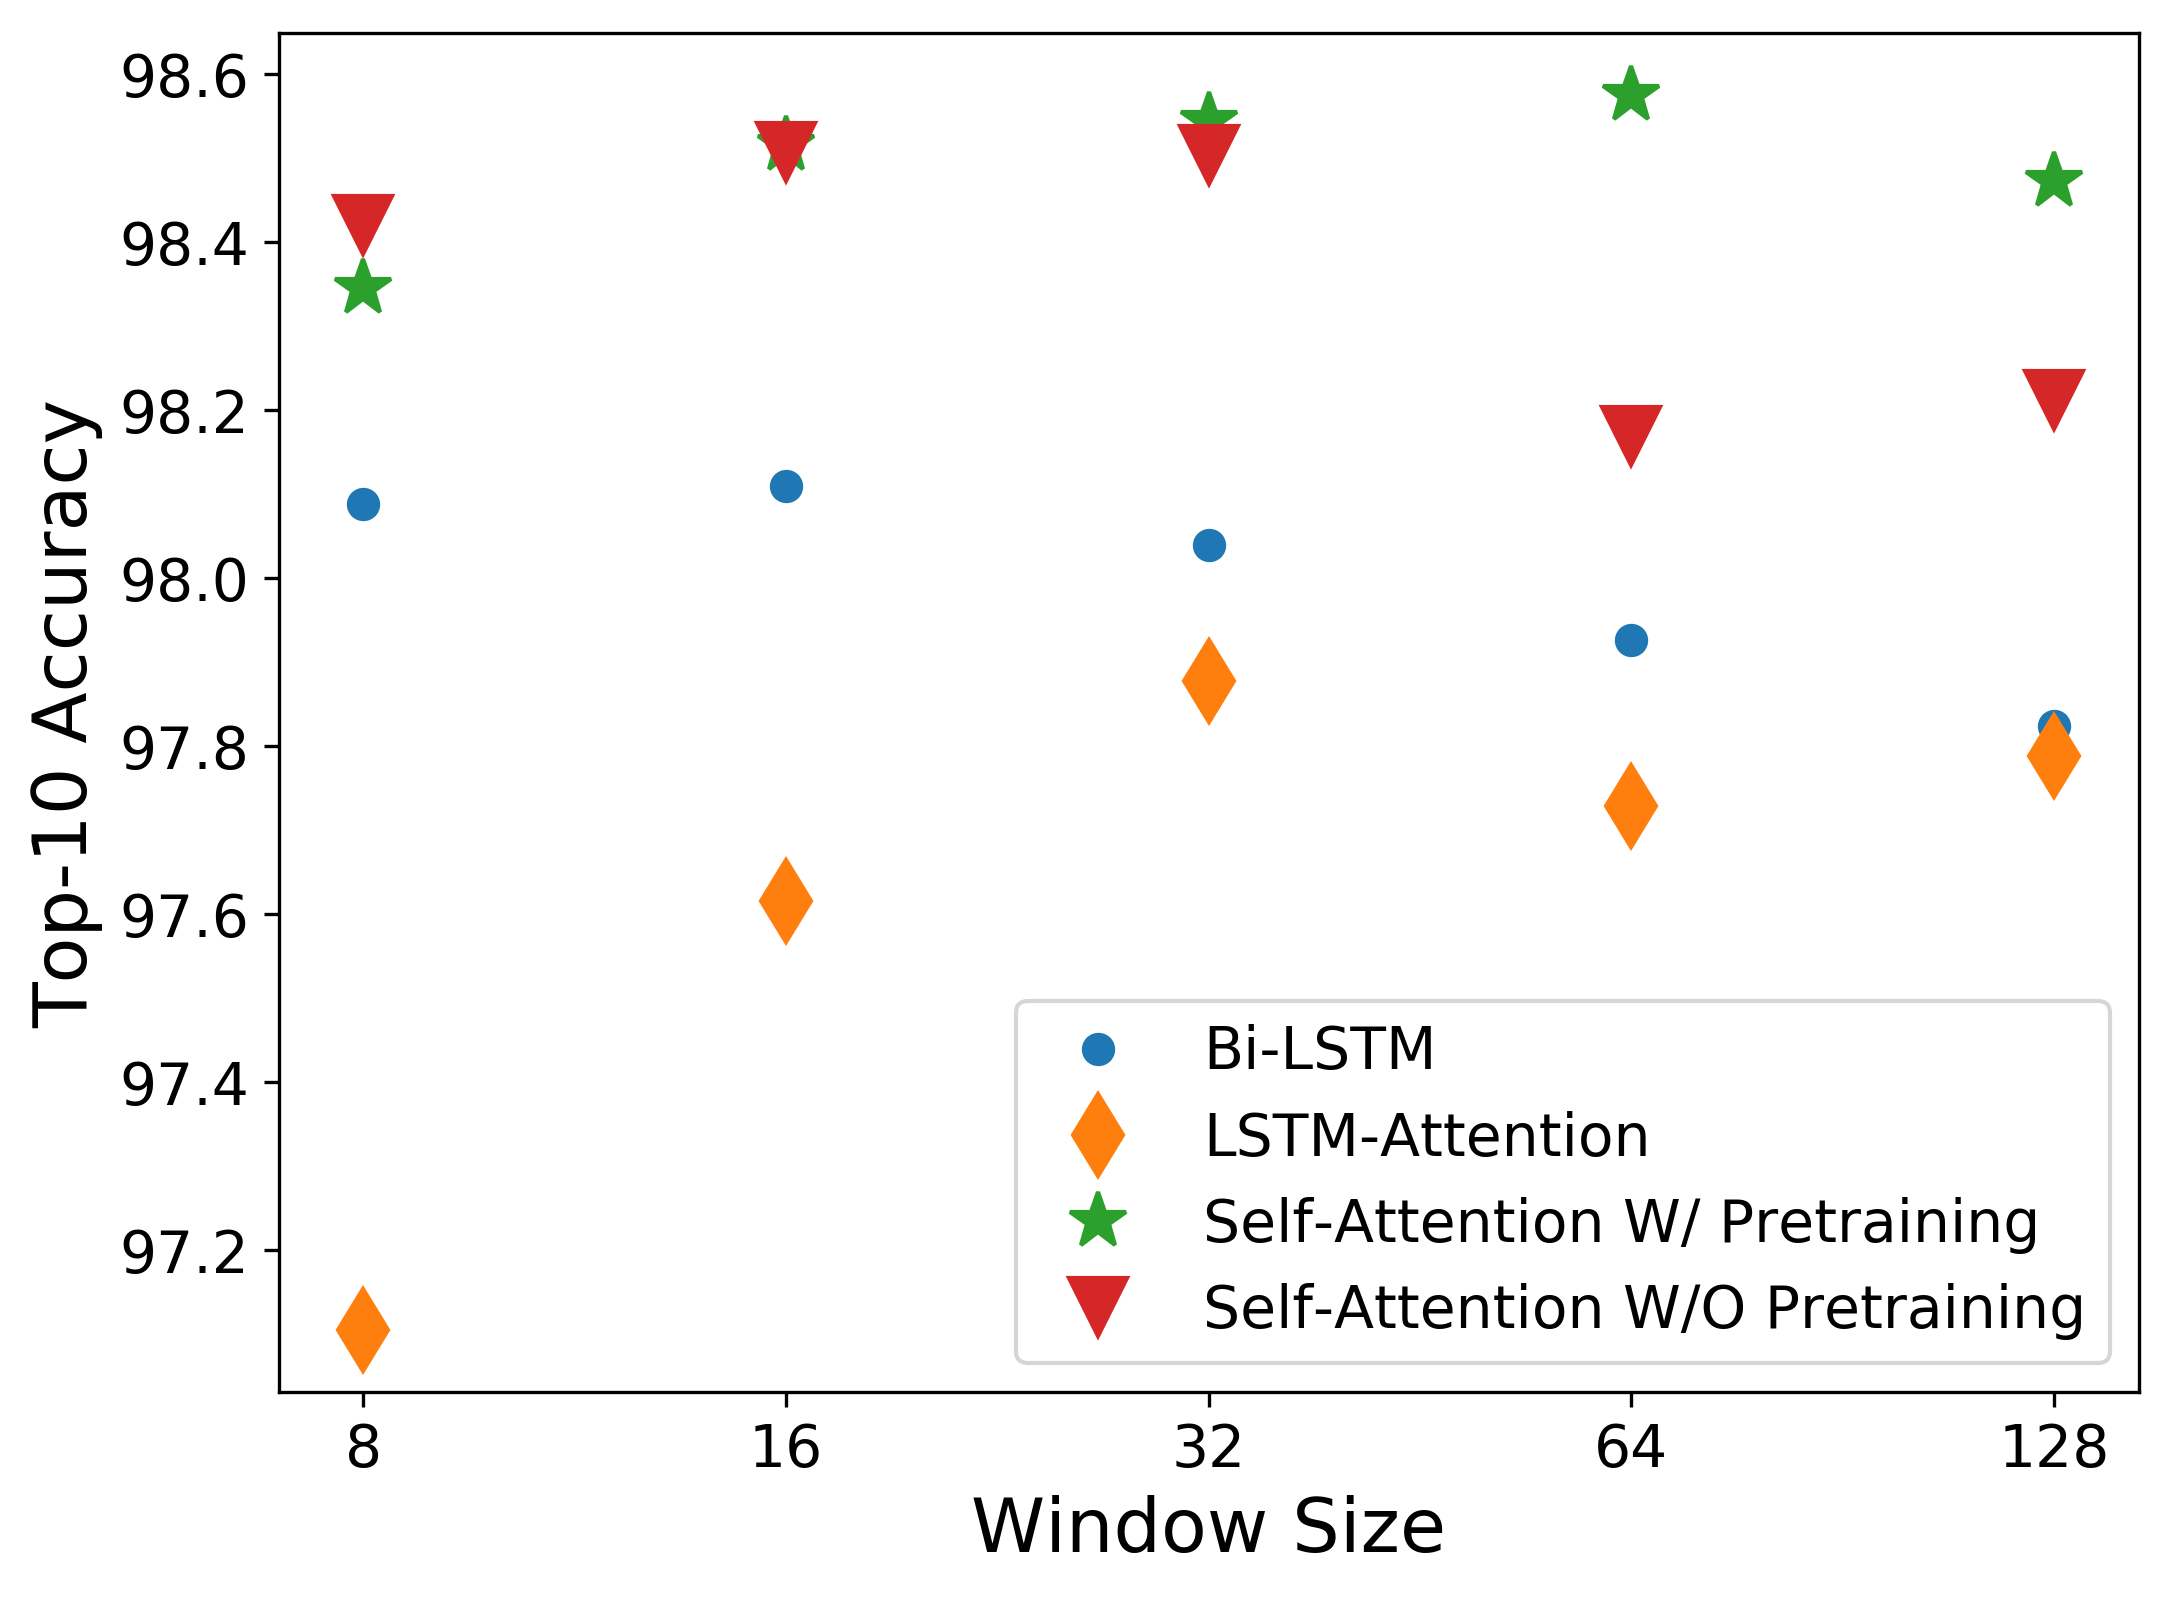}
\caption{DataAnalyzer2}
\end{subfigure}
\begin{subfigure}{0.32\linewidth}
\centering
\includegraphics[width=0.85\linewidth]{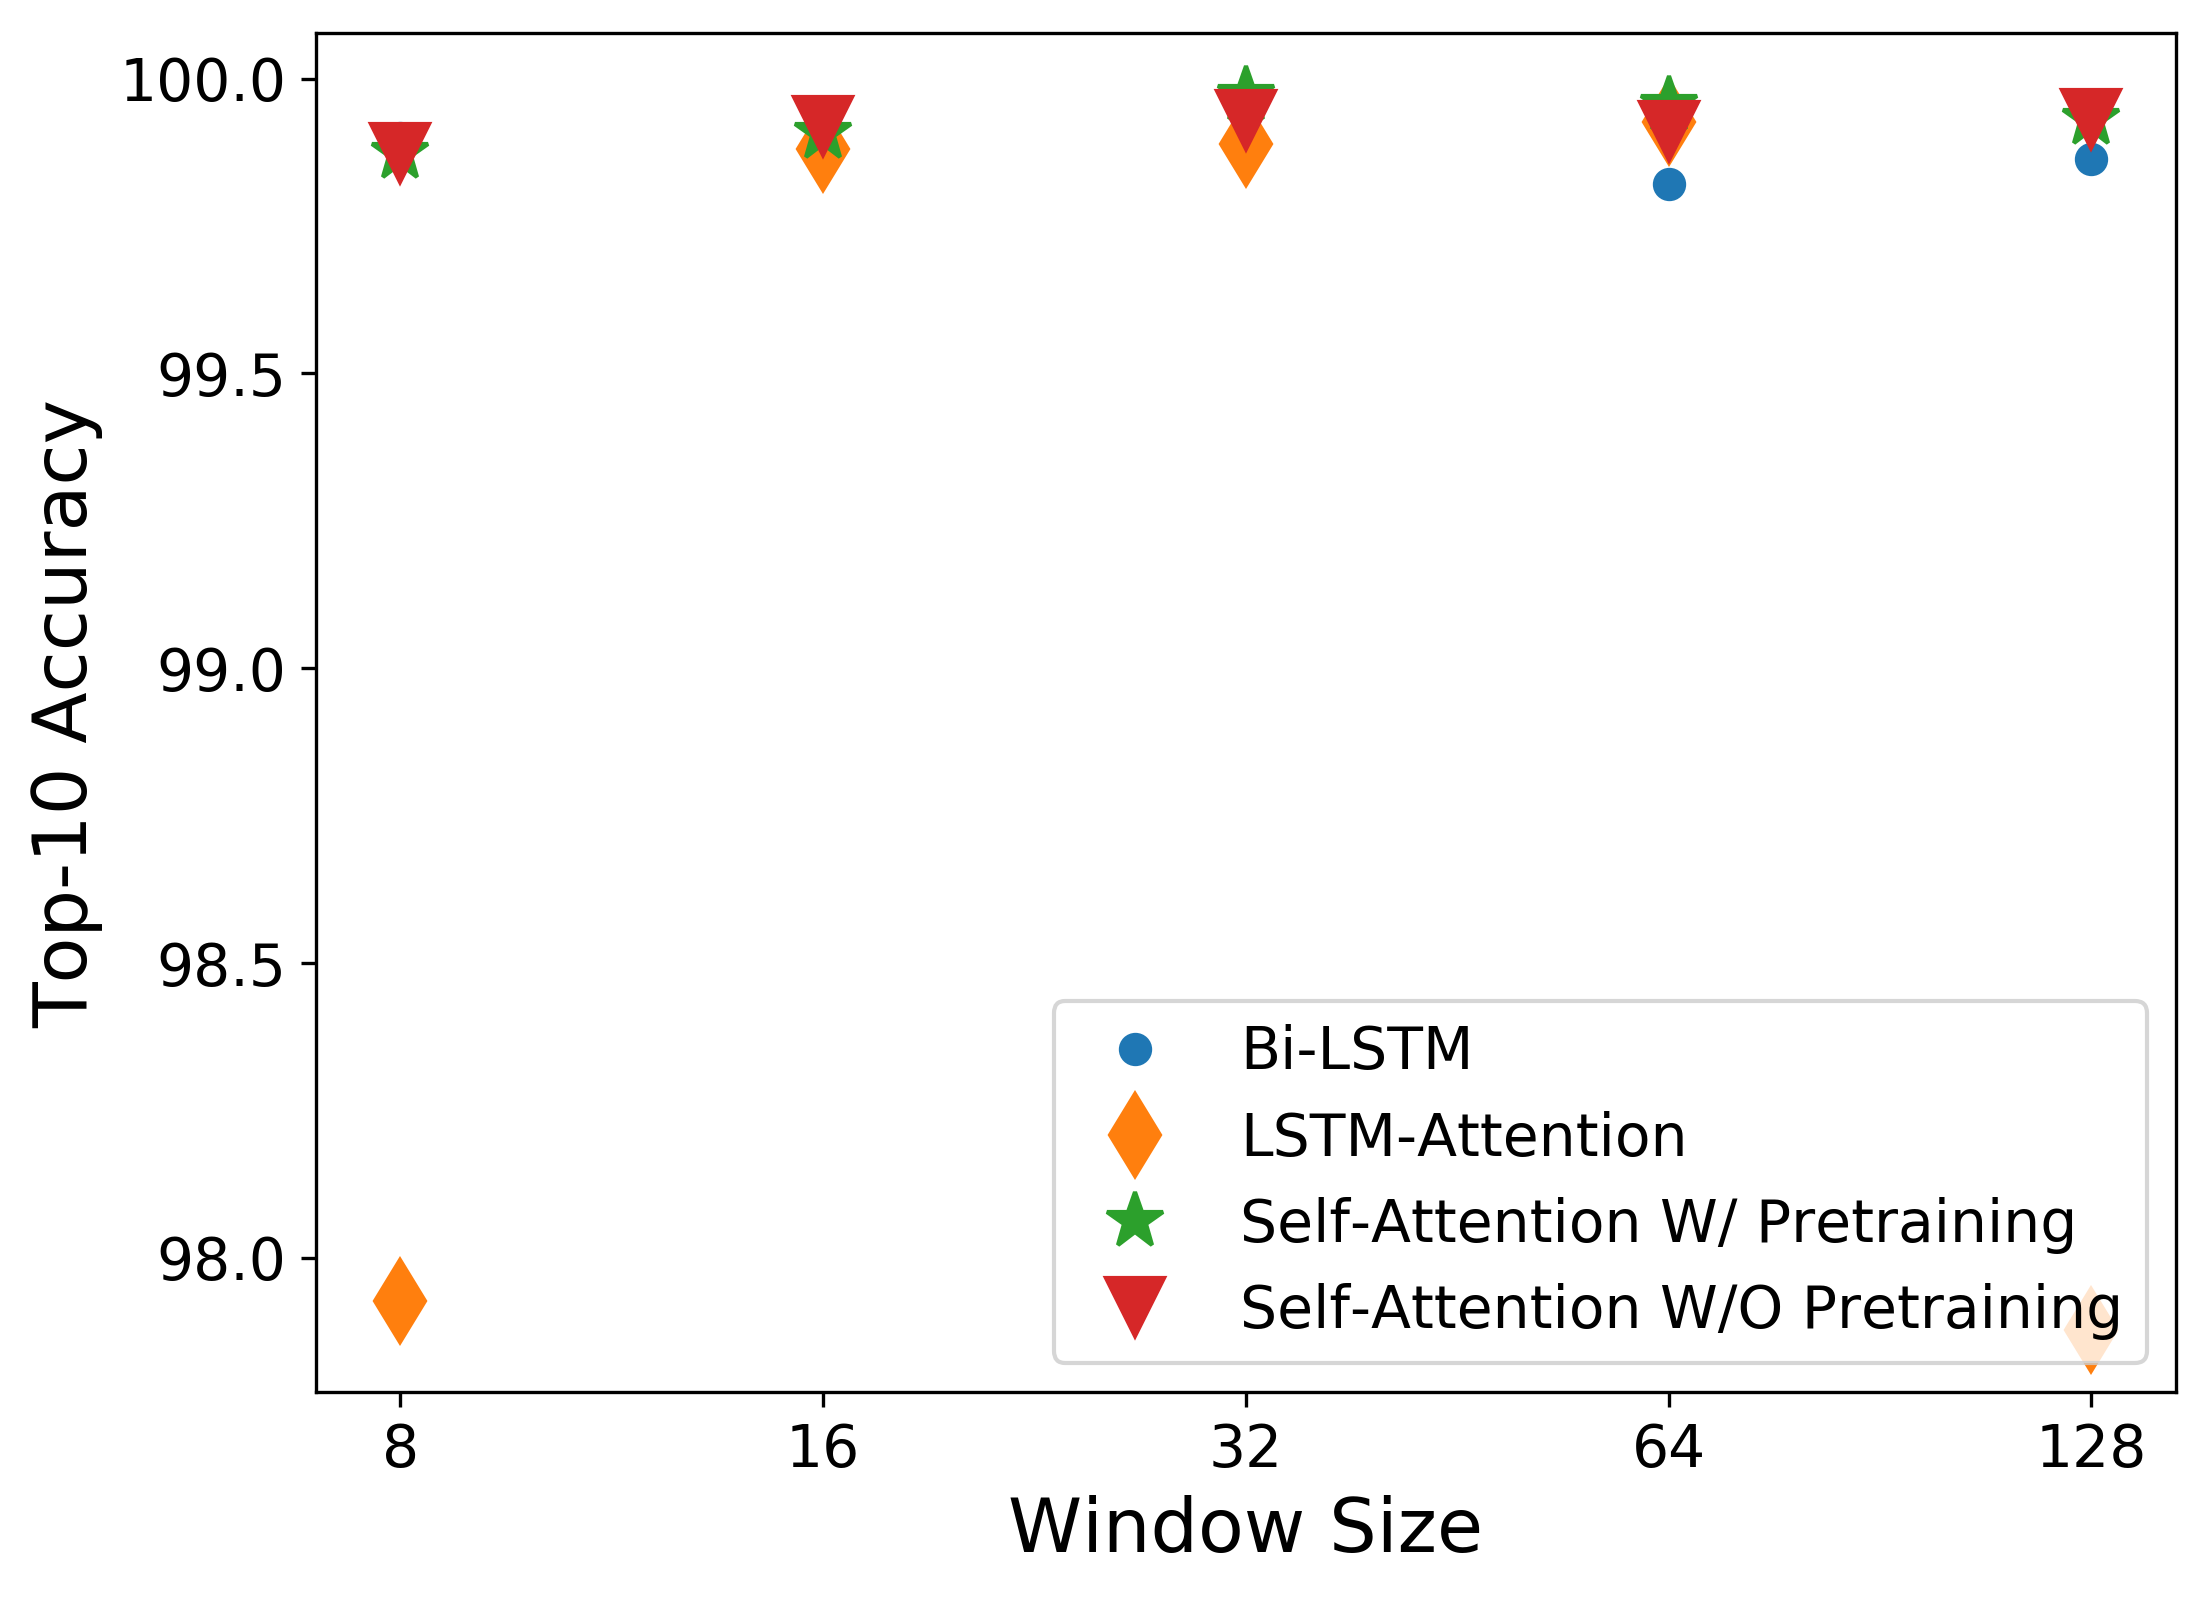}
\caption{DataRepo2}
\end{subfigure}
\caption{Model Comparison with Different Settings (Sequence Length and Pre-training) (Predicting Centered Events).}
\label{fig:setting_offline}
\end{figure*}
